# Supplementary material for: HI-PMK: A Data-Dependent Kernel for Incomplete Heterogeneous Data Representation
Source: arXiv:2501.04300 source file (2025-07-29)
Supplement: Supplementary file 1 [file supp.pdf]

# Supplementary Material for
# *HI-PMK: A Data-Dependent Kernel for Incomplete Heterogeneous Data Representation*

Youran Zhou*[1], Mohamed Reda Bouadjenek[1], Jonathan Wells[1], and Sunil Aryal[1]

[1]School of Information Technology, Deakin University, Australia

Supplementary material for the ECAI 2025 paper HI-PMK: A Data-Dependent Kernel for Incomplete Heterogeneous Data Representation[4].

## 1 Algorithms for HI-PMK Implementation

The supplementary algorithms detail the key computational steps for implementing the HI-PMK framework, designed to handle incomplete and heterogeneous datasets efficiently. **Algorithm 1** focuses on the pre-computation of bin data masses, where numerical features are discretized into bins, and missing values are systematically categorized into a dedicated bucket. This step ensures efficient probability mass calculations by leveraging pre-computed bin-level statistics. **Algorithm 2** and **Algorithm 3** extend the original PMK to handle incomplete data by addressing scenarios where one or both feature values are missing. These algorithms compute the adjusted probability mass for such cases, employing a conservative approach to maximize dissimilarity and ensure robustness under various missing mechanisms. Finally, **Algorithm 4** presents the overall computation of the Probability Mass Kernel (PMK), integrating the $m_0$-dissimilarity measure and normalization across all instance pairs. The modular structure of these algorithms allows flexibility in adapting HI-PMK to diverse data characteristics while ensuring computational efficiency and scalability. Each algorithm is complemented with clear notation and comments to enhance interpretability and facilitate reproducibility.

*Corresponding author: echo.zhou@deakin.edu.au

**Algorithm 1** Pre-computation of Bin Data Mass

**Require:** $\boldsymbol{X} \in \mathbb{R}^{n \times m}$: Dataset with $n$ samples and $m$ features
**Require:** $[b_i]$: Binning thresholds or hetero-states for discretization
**Ensure:** Pre-computed bin data masses for all features

```
for k = 1 to m do
    Initialize 𝓑_k ← ∅ {Bin for missing values}
    Initialize bins [B_i], i ∈ [1, b] {Bins for feature k}
    Discretize feature x_k using [b_i] or hetero-states
    for j = 1 to n do
        if x_k^(j) is not missing then
            Assign x_k^(j) to its corresponding bin B_i
        else
            Assign x_k^(j) to 𝓑_k {Handle missing values}
        end if
    end for
end for
return Pre-computed bin data masses for all features
```

**Algorithm 2** Adjust Probability Mass for Single Missing Value

**Require:** $x_k$: Observed value, '?': Missing value, $\mathcal{B}_k$: Bin for missing values
**Ensure:** Adjusted probability mass $|R_k(x_k, ?)|$

```
if k is numerical or ordinal then
    Compute 𝓜_L(x_k) and 𝓜_R(x_k)
    |R_k(x_k, ?)| ← max(𝓜_L(x_k), 𝓜_R(x_k)) + |𝓑_k|
else
    Compute 𝓜(x_k) and max_{a∈𝓢_k} 𝓜(a)
    |R_k(x_k, ?)| ← 𝓜(x_k) + max_{a∈𝓢_k} 𝓜(a) + |𝓑_k|
end if
return |R_k(x_k, ?)|
```

**Algorithm 3** Adjust Probability Mass for Both Missing Values

**Require:** Feature $k$: Numerical, ordinal, or nominal
**Require:** $\mathcal{B}_k$: Bin for missing values
**Ensure:** Adjusted probability mass $|R_k(?, ?)|$

```
if k is numerical or ordinal then
    |R_k(?, ?)| ← m {Total number of instances including missing values}
else
    Compute max_{a∈𝓢_k} 𝓜(a)
    |R_k(?, ?)| ← max_{a∈𝓢_k} 𝓜(a) + |𝓑_k|
end if
return |R_k(?, ?)|
```

**Algorithm 4** PMK Computation for Incomplete Data

**Require:** $\boldsymbol{X} \in \mathbb{R}^{n \times m}$: Dataset with $n$ samples and $m$ features
**Require:** Pre-computed bin data masses from Algorithm 1
**Ensure:** PMK similarity matrix for all instance pairs

```
Initialize m_0(x^(i), x^(j)) ← 0 for all i, j ∈ [1, n]
for i = 1 to n do
  for j = i to n do
    for k = 1 to m do
      if One of x_k^(i) or x_k^(j) is missing then
        Compute |R_k(x_k^(i), ?)| or |R_k(x_k^(j), ?)| using Algorithm 2
      else if Both x_k^(i) and x_k^(j) are missing then
        Compute |R_k(?, ?)| using Algorithm 3
      else
        Compute |R_k(x_k^(i), x_k^(j))| using pre-computed bin data masses
      end if
      Update m_0(x^(i), x^(j)) ← m_0(x^(i), x^(j)) + log( |R_k(x_k^(i), x_k^(j))| / n )
    end for
    Normalize m_0(x^(i), x^(j)) ← m_0(x^(i), x^(j)) / m
  end for
end for
Compute PMK using:
PMK(x^(i), x^(j)) ← 2×m_0(x^(i), x^(j)) / ( m_0(x^(i), x^(i)) + m_0(x^(j), x^(j)) )
return PMK matrix
```

In LaTeX form, the key steps are:

$m_0(\mathbf{x}^{(i)}, \mathbf{x}^{(j)}) \leftarrow m_0(\mathbf{x}^{(i)}, \mathbf{x}^{(j)}) + \log \frac{|R_k(x_k^{(i)}, x_k^{(j)})|}{n}$

$m_0(\mathbf{x}^{(i)}, \mathbf{x}^{(j)}) \leftarrow \frac{m_0(\mathbf{x}^{(i)}, \mathbf{x}^{(j)})}{m}$

$PMK(\mathbf{x}^{(i)}, \mathbf{x}^{(j)}) \leftarrow \frac{2 \times m_0(\mathbf{x}^{(i)}, \mathbf{x}^{(j)})}{m_0(\mathbf{x}^{(i)}, \mathbf{x}^{(i)}) + m_0(\mathbf{x}^{(j)}, \mathbf{x}^{(j)})}$

## 2 Complexity Analysis

**Overall Time Complexity:** The pairwise similarity computation for $m$ objects in an $n$-dimensional space with HI-PMK has a base time complexity of $O(m^2 \times n)$, which is comparable to traditional distance measures like Euclidean distance. This complexity arises from calculating pairwise similarities for all $m \times m$ object pairs across $n$ features.

**Pre-computation Phase:** The pre-computation of bin data masses (Algorithm 1) involves discretizing each feature into $b$ bins and handling missing values. The time complexity of this step is $O(n \times m)$, as each feature is iterated over all $m$ data points. Assuming $b$ is small compared to $m$, this phase introduces a negligible computational overhead relative to the overall algorithm.

**Handling Missing Data:** For incomplete data, the adjusted probability mass calculations in Algorithm 2 and Algorithm 3 depend on the number of missing values in the dataset. If the fraction of missing values per feature is $\rho$, the additional operations scale with $O(\rho \times m^2 \times n)$. The use of pre-computed bin data masses mitigates the computational cost, ensuring efficient lookups during pairwise similarity computation.

**Pairwise Similarity Computation:** The main computational cost comes from the pairwise similarity calculation (Algorithm 4), where $m^2$ pairs are evaluated across $n$ features. For each pair, the size of the region $|R_k(x_k^{(i)}, x_k^{(j)})|$ is retrieved from pre-computed data, reducing redundant computations. This step dominates the overall time complexity, resulting in $O(m^2 \times n)$.

**Space Complexity:** The primary space requirement is for storing the pairwise similarity matrix, which has a complexity of $O(m^2)$. Additionally, the storage of pre-computed bin data masses for all $n$ features requires $O(n \times b^2)$ space, where $b$ is the number of bins per feature. Since $b$ is typically much smaller than $m$, this storage overhead is minimal compared to the similarity matrix.

**Practical Considerations:** While the theoretical complexity of $O(m^2 \times n)$ may seem computationally expensive for large datasets, the use of pre-computed bin data masses significantly reduces redundant operations, improving practical runtime performance. Furthermore, the modular nature of the algorithm allows parallelization across features or instance pairs, which can further enhance efficiency on modern hardware.

## 3 Methodology Discussion

Table 1 presents the results of our detail compare study, which evaluates the impact of key components and alternative strategies in HI-PMK on both complete and incomplete datasets. The performance is reported across three missing mechanisms (MCAR, MAR, MNAR) for complete datasets and classification/clustering tasks for incomplete datasets.

### 3.1 Separate Bucket $\mathcal{B}_k$

To evaluate the necessity and effectiveness of the separate bucket $\mathcal{B}_k$, we conducted additional experiments where alternative strategies were employed to handle missing data. Specifically, we tested the following scenarios:

- **Random Assignment:** Missing values were randomly assigned to one of the regular bins used for discretizing observed data.
- **Mass-Based Assignment:** Missing values were assigned to the bin with the largest data mass ($\max_b \mathcal{M}_b$), assuming this bin represented the most probable range for missing values.

The results revealed that both alternative strategies introduced significant biases, leading to performance degradation across all evaluated datasets. For the **random assignment** strategy, the randomness disrupted the structure of observed data, causing inconsistencies in similarity computations. This random scattering of missing values failed to account for potential correlations between observed and missing values, particularly under MAR and MNAR mechanisms.

In contrast, the **mass-based assignment** strategy artificially concentrated missing values into the bin with the largest data mass. While this approach reduced randomness, it overestimated the likelihood of missing values belonging to a single range, particularly in datasets with skewed distributions. Consequently, this strategy distorted the feature distributions, negatively impacting downstream tasks such as classification and clustering.

The separate bucket $\mathcal{B}_k$ outperformed these alternatives in all scenarios. By isolating missing values, $\mathcal{B}_k$ ensured that their unique characteristics were preserved and explicitly modeled, avoiding the pitfalls of both random scattering and artificial concentration. This design aligns with theoretical principles of robust handling of incomplete data, as it minimizes the bias introduced by missing values while maintaining flexibility to model diverse missing mechanisms.

Empirical results highlight the superiority of $\mathcal{B}_k$, particularly under MNAR conditions where missing values often exhibit distinct patterns. The separate bucket allowed the framework to leverage these patterns, resulting in better similarity estimations and improved overall performance.

In conclusion, our experiments demonstrate that the separate bucket $\mathcal{B}_k$ is a critical component for robustly handling missing data. Alternative strategies, while simpler, fail to capture the complexities of real-world missingness and lead to suboptimal results. The design of $\mathcal{B}_k$ provides a theoretically sound and empirically validated approach to managing incomplete data, enhancing the adaptability and reliability of our framework.

### 3.2 Maximizing Uncertainty (MaxU)

The *Maximizing Uncertainty* (MaxU) strategy is a conservative dissimilarity estimation method rooted in the principle of maximum uncertainty [1]. It ensures robust inference by assigning the largest plausible dissimilarity to entries involving missing values, thereby avoiding overly optimistic similarity assumptions.

For numerical and ordinal features, MaxU assigns the maximum possible dissimilarity by considering the widest interval that a missing value could belong to, based on histogram-based binning. This effectively models the worst-case distributional uncertainty without requiring imputation. For nominal features, MaxU assumes the missing value could correspond to the most frequent or most dissimilar category, thus maximizing categorical distance. This mechanism-aware strategy is particularly suited for complex missingness patterns—such as those found under MNAR—where the underlying value distribution is not ignorable.

**Alternative Strategies.** To contextualize the benefit of MaxU, we compare it with two alternative uncertainty modeling approaches:

**(1) Average Uncertainty (AvgU):** This method estimates dissimilarity by averaging over all observed values, computing $|R_k(x_k, ?)|$ as the expected dissimilarity between the observed entry $x_k$ and the empirical value distribution. While moderate, AvgU may underestimate the variability in heavy-tailed or skewed distributions, leading to reduced robustness under non-random missingness.

**(2) Minimum Uncertainty (MinU):** This optimistic variant assumes the missing value is most similar to the known value $x_k$, minimizing $|R_k(x_k, ?)|$. Although it yields smaller dissimilarities, MinU is prone to overconfidence and fragile under adversarial or MNAR patterns.

**Empirical Findings.** As shown in Table 1, MaxU consistently outperforms AvgU and MinU across both complete and incomplete datasets. For example, in classification tasks on incomplete data, HI-PMK with MaxU achieves an F1 score of 0.8687, compared to 0.8597 for AvgU and 0.8417 for MinU. This confirms the value of MaxU in preserving discriminative capacity under uncertainty, particularly when the missingness mechanism is unknown or complex.

MaxU plays a pivotal role in HI-PMK by safeguarding against underestimation of dissimilarity. Its conservative nature enhances generalization and robustness across diverse scenarios, aligning with the minimax principle in robust statistics [2], which advocates pessimistic modeling under uncertainty to ensure worst-case resilience.

[1] Klir, G. J. (1995). *Principles of uncertainty: What are they? Why do we need them?* Fuzzy Sets and Systems, 74(1), 15–31.

| Dataset | Complete Datasets | | | Incomplete Datasets | |
|---|---|---|---|---|---|
| Type | MCAR | MAR | MNAR | Classification | Cluster |
| HI-PMK-Max | 0.5853 | 0.6175 | 0.5997 | 0.8544 | 0.3501 |
| HI-PMK-Rand | 0.6117 | 0.5975 | 0.5797 | 0.8518 | 0.3493 |
| HI-PMK-$\mathcal{B}$ | 0.6303 | 0.6510 | 0.6465 | 0.8687 | 0.3616 |
| HI-PMK-AvgU | 0.6215 | 0.6160 | 0.6031 | 0.8597 | 0.3591 |
| HI-PMK-MinU | 0.5920 | 0.5865 | 0.5933 | 0.8417 | 0.3117 |
| HI-PMK-MaxU | 0.6303 | 0.6510 | 0.6465 | 0.8687 | 0.3616 |

Table 1: Ablation study results

# 4 Implementation Details

## 4.1 Implementation

The source code for HI-PMK is publicly available at: Here. The framework was implemented in Python with computationally intensive components optimized using `C++`. Key libraries include `NumPy` for numerical computations and `scikit-learn` for evaluation metrics.

## 4.2 Parameter Settings

- **Number of bins ($b$):** The default number of bins for numerical features was initially determined using the formula: $b = \lfloor \log_2(\text{num\_instances}) \rfloor + 1$. However, in our experiments, $b$ was treated as a hyperparameter and carefully tuned for each dataset to optimize performance, ensuring the best representation of numerical features. We adopt Equal-Frequency (EF) binning with the number of bins $b$ chosen from a candidate set $\{20, 40, 60, 80, 100, \log_2(m)\}$, following classical binning heuristics [3] and practices from prior work on histogram-based similarity kernels [1].
- **Numerical Features:** Equal-frequency discretization was applied to divide the feature values into $b$ bins.
- **Categorical Features:** Probabilities of categorical labels were directly computed from their frequencies in the dataset.
- **Missing Data:** Missing values were handled using a bucket-based representation ($\mathcal{B}_k$) combined with the Maximum Uncertainty (MaxU) strategy to ensure robustness under various missing mechanisms.

### 4.3 Baselines

To evaluate the performance of HI-PMK, we compared it against the following baseline methods:

- **genRBF:** A similarity-based kernel method specifically designed for incomplete data. [Repository]
- **MissForest:** A tree-based imputation method implemented using the `missingpy` library. [Documentation]
- **GAIN:** A GAN-based imputation method implemented using the official TensorFlow code. [Repository]
- **MICE:** A widely used multiple imputation method for handling missing data.
- **MEAN:** A simple imputation baseline that fills missing values with feature-wise means.
- **KPCA:** Kernel Principal Component Analysis implemented using `scikit-learn`.
- **PPCA:** Probabilistic Principal Component Analysis implemented using the `ppca` library. [Documentation]

### 4.4 Dataset

Below are the links to the datasets used in our experiments:

- CAR Evaluation Dataset
- Breast Cancer Dataset
- Australian Credit Dataset
- Heart Disease Dataset
- Adult Dataset
- Student Performance Dataset
- Banknote Authentication Dataset
- Sonar Dataset
- Spam Dataset
- Wine Quality Dataset

## 4.5 Missing Data Generation

In our experiments, we generated missing data for the complete datasets under three different mechanisms: *Missing Completely at Random (MCAR)*, *Missing at Random (MAR)*, and *Missing Not at Random (MNAR)*. We evaluated the model's performance across nine missing rates: 5%, 10%, 20%, 30%, 40%, 50%, 60%, 70%, and 80%. The following subsections provide a detailed description of the missing data generation process for each mechanism.

### 4.5.1 MCAR Generation

For MCAR, missing values were introduced by randomly removing data points from the dataset. This process ensures that the probability of a value being missing is independent of its own value and other feature values. Specifically:

- For each feature, a uniform random selection process was applied to remove data points.
- This method simulates scenarios where missing data occurs without any inherent bias (e.g., accidental deletion or random dropout during data collection).

### 4.5.2 MAR Generation

For MAR, missing values were generated based on the values of other features in the dataset. The process is described as follows:

- A target feature $x_k$ was selected, and an auxiliary feature $x_{k'}$ was chosen to control the missingness in $x_k$.
- Missing values in $x_k$ were introduced for instances where $x_{k'}$ exceeded or fell below a threshold (e.g., mean, median, or percentile value).
- The dependency between $x_k$ and $x_{k'}$ was randomly assigned or derived from known correlations when available.

This process mirrors real-world cases where missing data in one feature is influenced by another feature, such as income data missing based on education level.

### 4.5.3 MNAR Generation

Generating MNAR data is more complex, as missingness depends on the unobserved value itself. We implemented a column-wise MNAR generation strategy with the following steps:

**Numerical Features:**

- A percentile threshold was computed for each numerical feature.
- Values above or below this threshold were selectively removed. For instance, values within the bottom 10% or top 10% of the feature range were made missing.
- This approach simulates scenarios where extreme values (e.g., sensor outliers) are more prone to being missing.

**Ordinal Features:**

- Missing values were biased towards extreme categories (e.g., the highest or lowest values in ordinal data such as satisfaction levels).
- Categories closer to the mean were less likely to have missing values.

**Nominal Features:**

- A specific category was selected with a higher probability of being missing. For example, in a color dataset, "Red" might be chosen as the category with a higher missing rate.
- If the target missing rate was not achieved by removing values from the selected category, additional categories were randomly sampled to ensure the desired overall missing rate was met.

### 4.6 Missing Rates

For all three mechanisms (MCAR, MAR, MNAR), missing data was generated at the following rates:

- 5%, 10%, 20%, 30%, 40%, 50%, 60%, 70%, and 80%.

### 4.7 Evaluation Metrics

To ensure a comprehensive evaluation of HI-PMK across different tasks and datasets, we utilized the following metrics:

- **Classification Tasks:** For incomplete datasets, which primarily involve binary classification tasks, we evaluated performance using both **accuracy** and **F1 scores**, as these metrics effectively capture the balance between precision and recall. For complete datasets, which often include multi-class classification tasks, we primarily used **F1 scores** to account for the class imbalance and provide a more nuanced evaluation of model performance.
- **Clustering Tasks:** To assess the quality of clustering, we employed **Normalized Mutual Information (NMI)** and **Adjusted Rand Index (ARI)**. These metrics quantify the alignment between predicted clusters and ground truth labels, offering complementary perspectives on clustering quality.

# 5 Implementation Details of Scalability Experiments

## Hardware and Software Configuration

All scalability experiments were conducted on a local workstation with the following configuration:

- **CPU:** Intel Core i7-13700KF @ 3.40GHz (13th Gen, 16 cores, 24 threads)
- **RAM:** 32 GB
- **GPU:** NVIDIA GeForce RTX 4070 Ti (used only for GAIN and other deep models)

## Synthetic Data Generation

To evaluate runtime scalability under controlled conditions, we generated synthetic tabular datasets with the following configurable parameters:

- **Sample Size** (`d`): Number of rows (data points).
- **Feature Dimension** (`n`): Number of columns (features).
- **Missing Rate** (`r`): Proportion of missing values, simulated under the MCAR (Missing Completely at Random) mechanism.

Data was generated using `sklearn.datasets.make_classification()`, followed by MCAR injection via random masking:

```
missing_mask = rng.uniform(0, 1, size=X.shape) < missing_rate
X[missing_mask] = np.nan
```

## Experimental Protocol

We tested three scalability dimensions:

- **Sample Size Scaling:** Fixed feature dimension ($n = 30$), varying $d \in \{500, 1000, 2000\}$, at 30% missing rate.
- **Feature Dimension Scaling:** Fixed sample size ($d = 1000$), varying $n \in \{100, 500, 1000\}$, at 30% missing rate.
- **Missing Rate Scaling:** Fixed $d = 30$, $n = 1000$, varying missing rate in $\{10\%, 30\%, 50\%\}$.

Each experiment was repeated 5 times. We recorded the average runtime and standard deviation of each method using Python's `time.time()` function, covering both kernel computation (e.g., HI-PMK) and model runtime (e.g., GAIN).

# 6 Complete Result Tables

In this section, we provide detailed result tables for all datasets, including metrics such as average accuracy, F1 scores, Normalized Mutual Information (NMI), and Adjusted Rand Index (ARI), along with their respective standard deviations (Std). These results are presented for both incomplete and complete datasets to comprehensively evaluate the performance of our proposed method.

## 6.1 Results for Incomplete Datasets

The results for classification tasks on incomplete datasets are summarized in the following tables:

- Table 2 presents the average accuracy and corresponding standard deviations across all datasets.
- Table 3 provides the average F1 scores and their standard deviations for classification tasks.

For clustering tasks on incomplete datasets, we include:

- Table 4 summarizes the Normalized Mutual Information (NMI) scores along with standard deviations.
- Table 5 presents the Adjusted Rand Index (ARI) values with their standard deviations.

## 6.2 Results for Complete Datasets

To evaluate performance on complete datasets, we provide the following:

- Table 6 reports the average F1 scores with standard deviations for classification tasks.

Detailed results for various missing rate for each dataset are available in the following tables:

- Table 7: Average F1 scores for the Australian dataset.
- Table 8: Average F1 scores for the Banknote dataset.
- Table 9: Average F1 scores for the Breast Cancer dataset.
- Table 10: Average F1 scores for the Car dataset.
- Table 13: Average F1 scores for the Spam dataset.
- Table 15: Average F1 scores for the Wine dataset.
- Table 11: Average F1 scores for the Heart dataset.

| **Method** | Hepat | Horse | Kidney | Mammo | Pima | Wiscon |
|---|---|---|---|---|---|---|
| Mean | $0.8129_{\pm 0.0747}$ | $0.8398_{\pm 0.0295}$ | $0.9775_{\pm 0.0200}$ | $0.8148_{\pm 0.0350}$ | $0.7735_{\pm 0.0205}$ | $0.9628_{\pm 0.0152}$ |
| MICE | $0.8129_{\pm 0.0718}$ | $0.8506_{\pm 0.0328}$ | $0.9700_{\pm 0.0170}$ | $0.8241_{\pm 0.0392}$ | $0.7722_{\pm 0.0180}$ | $0.9614_{\pm 0.0154}$ |
| EM | $0.8000_{\pm 0.0658}$ | $0.8398_{\pm 0.0438}$ | $0.9500_{\pm 0.0262}$ | $0.8200_{\pm 0.0404}$ | $0.7696_{\pm 0.0247}$ | $0.9614_{\pm 0.0184}$ |
| Mis | $0.8065_{\pm 0.0540}$ | $0.8262_{\pm 0.0370}$ | $0.9650_{\pm 0.0094}$ | $0.8200_{\pm 0.0390}$ | $0.7722_{\pm 0.0167}$ | $0.9628_{\pm 0.0152}$ |
| GAIN | $0.8274_{\pm 0.0241}$ | $0.8561_{\pm 0.0374}$ | $0.8525_{\pm 0.1166}$ | $0.8106_{\pm 0.0331}$ | $0.7462_{\pm 0.0401}$ | $0.9642_{\pm 0.0163}$ |
| genRBF | $0.7935_{\pm 0.0158}$ | $0.6304_{\pm 0.0049}$ | $0.6250_{\pm 0.0000}$ | $0.5140_{\pm 0.0139}$ | $0.6510_{\pm 0.0021}$ | $0.5564_{\pm 0.0429}$ |
| KPCA | $0.7935_{\pm 0.0158}$ | $0.6850_{\pm 0.0389}$ | $0.6250_{\pm 0.0000}$ | $0.8127_{\pm 0.0249}$ | $0.6510_{\pm 0.0021}$ | $0.9500_{\pm 0.0313}$ |
| PPCA | $0.8000_{\pm 0.0718}$ | $0.8506_{\pm 0.0307}$ | $0.9625_{\pm 0.0274}$ | $0.8241_{\pm 0.0392}$ | $0.7722_{\pm 0.0180}$ | $0.9628_{\pm 0.0152}$ |
| HI-PMK | $0.8065_{\pm 0.0353}$ | $0.8506_{\pm 0.8127}$ | $0.9875_{\pm 0.9868}$ | $0.8221_{\pm 0.8157}$ | $0.7735_{\pm 0.0312}$ | $0.9700_{\pm 0.0165}$ |

Table 2: Average accuracy and standard deviation across datasets for classification tasks on incomplete data.

| **Method** | Hepat | Horse | Kidney | Mammo | Pima | Wiscon |
|---|---|---|---|---|---|---|
| Mean | $0.6991_{\pm 0.0900}$ | $0.8262_{\pm 0.0312}$ | $0.9761_{\pm 0.0213}$ | $0.8095_{\pm 0.0404}$ | $0.7324_{\pm 0.0234}$ | $0.9589_{\pm 0.0169}$ |
| MICE | $0.6938_{\pm 0.0864}$ | $0.8371_{\pm 0.0357}$ | $0.9682_{\pm 0.0181}$ | $0.8196_{\pm 0.0454}$ | $0.7317_{\pm 0.0200}$ | $0.9574_{\pm 0.0170}$ |
| EM | $0.6617_{\pm 0.1159}$ | $0.8256_{\pm 0.0455}$ | $0.9471_{\pm 0.0281}$ | $0.8155_{\pm 0.0460}$ | $0.7285_{\pm 0.0234}$ | $0.9573_{\pm 0.0206}$ |
| MisF | $0.6666_{\pm 0.1265}$ | $0.8107_{\pm 0.0407}$ | $0.9631_{\pm 0.0097}$ | $0.8155_{\pm 0.0449}$ | $0.7306_{\pm 0.0181}$ | $0.9589_{\pm 0.0169}$ |
| GAIN | $0.5918_{\pm 0.0621}$ | $0.8450_{\pm 0.0377}$ | $0.8101_{\pm 0.1690}$ | $0.8047_{\pm 0.0384}$ | $0.7034_{\pm 0.0653}$ | $0.9605_{\pm 0.0181}$ |
| genRBF | $0.4424_{\pm 0.0049}$ | $0.3867_{\pm 0.0019}$ | $0.3846_{\pm 0.0000}$ | $0.5123_{\pm 0.0145}$ | $0.3943_{\pm 0.0008}$ | $0.5024_{\pm 0.0355}$ |
| KPCA | $0.4424_{\pm 0.0049}$ | $0.5667_{\pm 0.0554}$ | $0.3846_{\pm 0.0000}$ | $0.8116_{\pm 0.0257}$ | $0.3943_{\pm 0.0008}$ | $0.9463_{\pm 0.0330}$ |
| PPCA | $0.6865_{\pm 0.0728}$ | $0.8363_{\pm 0.0334}$ | $0.9602_{\pm 0.0290}$ | $0.8196_{\pm 0.0454}$ | $0.7317_{\pm 0.0200}$ | $0.9589_{\pm 0.0169}$ |
| HI-PMK | $0.6959_{\pm 0.0514}$ | $0.8217_{\pm 0.0194}$ | $0.9777_{\pm 0.0145}$ | $0.8298_{\pm 0.0364}$ | $0.7327_{\pm 0.0312}$ | $0.9607_{\pm 0.0182}$ |

Table 3: Average F1 scores and standard deviation for classification tasks on incomplete data.

| Method | Hepat | Horse | Kidney | Mammo | Pima | Wiscon |
|---|---|---|---|---|---|---|
| Mean | $0.0015_{\pm 0.0000}$ | $0.0078_{\pm 0.0000}$ | $0.0067_{\pm 0.0000}$ | $0.0959_{\pm 0.0000}$ | $0.0111_{\pm 0.0000}$ | $0.7295_{\pm 0.0000}$ |
| MICE | $0.0021_{\pm 0.0012}$ | $0.0024_{\pm 0.0000}$ | $0.0074_{\pm 0.0000}$ | $0.0959_{\pm 0.0000}$ | $0.0910_{\pm 0.0000}$ | $0.7427_{\pm 0.0000}$ |
| EM | $0.0025_{\pm 0.0019}$ | $0.0079_{\pm 0.0023}$ | $0.0045_{\pm 0.0017}$ | $0.0911_{\pm 0.0011}$ | $0.0211_{\pm 0.0050}$ | $0.7387_{\pm 0.0033}$ |
| MisF | $0.0014_{\pm 0.0002}$ | $0.0078_{\pm 0.0000}$ | $0.0023_{\pm 0.0025}$ | $0.0959_{\pm 0.0000}$ | $0.0169_{\pm 0.0000}$ | $0.7335_{\pm 0.0032}$ |
| GAIN | $0.0012_{\pm 0.0004}$ | $0.0071_{\pm 0.0011}$ | $0.0160_{\pm 0.0115}$ | $0.0932_{\pm 0.0033}$ | $0.0569_{\pm 0.0153}$ | $0.7387_{\pm 0.0033}$ |
| genRBF | $0.0772_{\pm 0.0052}$ | $0.0166_{\pm 0.0000}$ | $0.0132_{\pm 0.0000}$ | $0.0002_{\pm 0.0000}$ | $0.0052_{\pm 0.0004}$ | $0.4505_{\pm 0.0000}$ |
| KPCA | $0.0159_{\pm 0.0226}$ | $0.0583_{\pm 0.0175}$ | $0.0056_{\pm 0.0065}$ | $0.0117_{\pm 0.0111}$ | $0.0092_{\pm 0.0115}$ | $0.5186_{\pm 0.0672}$ |
| PPCA | $0.0015_{\pm 0.0000}$ | $0.0540_{\pm 0.0047}$ | $0.0081_{\pm 0.0015}$ | $0.0959_{\pm 0.0000}$ | $0.0909_{\pm 0.0001}$ | $0.7427_{\pm 0.0000}$ |
| Simple | $0.0019_{\pm 0.0012}$ | $0.0001_{\pm 0.0001}$ | $0.0424_{\pm 0.0050}$ | $0.0951_{\pm 0.0017}$ | $0.0556_{\pm 0.0021}$ | $0.0000_{\pm 0.0000}$ |
| Gower | $0.1968_{\pm 0.0000}$ | $0.1280_{\pm 0.0000}$ | $0.3899_{\pm 0.0000}$ | $0.2970_{\pm 0.0000}$ | $0.1069_{\pm 0.0032}$ | $0.6939_{\pm 0.0000}$ |
| HI-PMK | $0.2001_{\pm 0.0055}$ | $0.1066_{\pm 0.0000}$ | $0.6663_{\pm 0.0000}$ | $0.3240_{\pm 0.0000}$ | $0.1244_{\pm 0.0039}$ | $0.7585_{\pm 0.0025}$ |

Table 4: Average Normalized Mutual Information (NMI) and standard deviation for clustering tasks on incomplete data.

| Method | Hepat | Horse | Kidney | Mammo | Pima | Wiscon |
|---|---|---|---|---|---|---|
| Mean | $0.1198_{\pm 0.0000}$ | $0.1262_{\pm 0.0000}$ | $0.2485_{\pm 0.0000}$ | $0.1133_{\pm 0.0000}$ | $0.0300_{\pm 0.0000}$ | $0.8337_{\pm 0.0000}$ |
| MICE | $0.1234_{\pm 0.0072}$ | $0.1110_{\pm 0.0000}$ | $0.3184_{\pm 0.0013}$ | $0.1133_{\pm 0.0000}$ | $0.1625_{\pm 0.0000}$ | $0.8444_{\pm 0.0000}$ |
| EM | $0.1248_{\pm 0.0099}$ | $0.1253_{\pm 0.0053}$ | $0.3243_{\pm 0.0017}$ | $0.1083_{\pm 0.0011}$ | $0.0572_{\pm 0.0086}$ | $0.8412_{\pm 0.0026}$ |
| MissForest | $0.1191_{\pm 0.0016}$ | $0.1262_{\pm 0.0000}$ | $0.3498_{\pm 0.0040}$ | $0.1133_{\pm 0.0000}$ | $0.0403_{\pm 0.0000}$ | $0.8369_{\pm 0.0026}$ |
| GAIN | $0.1170_{\pm 0.0034}$ | $0.1244_{\pm 0.0028}$ | $0.4069_{\pm 0.0132}$ | $0.1106_{\pm 0.0034}$ | $0.1074_{\pm 0.0254}$ | $0.8412_{\pm 0.0026}$ |
| genRBF | $0.1834_{\pm 0.0034}$ | $0.1044_{\pm 0.0000}$ | $0.4077_{\pm 0.0000}$ | $0.0007_{\pm 0.0000}$ | $0.0208_{\pm 0.0010}$ | $0.5390_{\pm 0.0000}$ |
| KPCA | $0.1394_{\pm 0.0312}$ | $0.1060_{\pm 0.0284}$ | $0.4051_{\pm 0.0123}$ | $0.0138_{\pm 0.0135}$ | $0.0137_{\pm 0.0115}$ | $0.5001_{\pm 0.1082}$ |
| PPCA | $0.1198_{\pm 0.0000}$ | $0.1250_{\pm 0.0052}$ | $0.4193_{\pm 0.0004}$ | $0.1133_{\pm 0.0000}$ | $0.1621_{\pm 0.0004}$ | $0.8444_{\pm 0.0000}$ |
| Simple | $0.1127_{\pm 0.0064}$ | $0.1030_{\pm 0.0010}$ | $0.3237_{\pm 0.0024}$ | $0.1101_{\pm 0.0066}$ | $0.0998_{\pm 0.0034}$ | $0.0000_{\pm 0.0000}$ |
| Gower | $0.2115_{\pm 0.0000}$ | $0.1341_{\pm 0.0000}$ | $0.6880_{\pm 0.0000}$ | $0.3548_{\pm 0.0000}$ | $0.1753_{\pm 0.0038}$ | $0.8020_{\pm 0.0000}$ |
| HI-PMK | $0.1958_{\pm 0.0313}$ | $0.1434_{\pm 0.0000}$ | $0.7048_{\pm 0.0000}$ | $0.3827_{\pm 0.0000}$ | $0.1992_{\pm 0.0059}$ | $0.8445_{\pm 0.0026}$ |

Table 5: Average Adjusted Rand Index (ARI) and standard deviation for clustering tasks on incomplete data.

| Model | Adult | Australian | Banknote | Breast | Car | Heart | Sonar | Spam | Student | Wine |
|---|---|---|---|---|---|---|---|---|---|---|
| **MCAR** | | | | | | | | | | |
| Mean | 0.2546 ± 0.0022 | 0.6127 ± 0.0394 | 0.7619 ± 0.0205 | 0.4278 ± 0.0007 | 0.4377 ± 0.0265 | 0.1774 ± 0.0009 | 0.6912 ± 0.0519 | 0.6978 ± 0.0183 | 0.1985 ± 0.0295 | 0.7962 ± 0.0108 |
| MICE | 0.2178 ± 0.0033 | 0.6123 ± 0.0399 | 0.7725 ± 0.0165 | 0.4508 ± 0.0007 | 0.4285 ± 0.0278 | 0.1774 ± 0.0009 | 0.7406 ± 0.0545 | 0.6933 ± 0.0170 | 0.2126 ± 0.0327 | 0.8563 ± 0.0090 |
| EM | 0.2269 ± 0.0042 | 0.4800 ± 0.0455 | 0.7709 ± 0.0216 | 0.4515 ± 0.0007 | 0.3736 ± 0.0177 | 0.1774 ± 0.0009 | 0.6628 ± 0.0438 | 0.5148 ± 0.0262 | 0.1742 ± 0.0134 | 0.6900 ± 0.0105 |
| MisF | 0.2584 ± 0.0545 | 0.6909 ± 0.0286 | 0.8109 ± 0.0157 | 0.4160 ± 0.0037 | 0.3741 ± 0.0255 | 0.2281 ± 0.0274 | 0.6977 ± 0.0508 | 0.5694 ± 0.0241 | 0.1660 ± 0.0297 | 0.9234 ± 0.0087 |
| GAIN | 0.2423 ± 0.0033 | 0.7547 ± 0.0257 | 0.7613 ± 0.0229 | 0.4135 ± 0.0021 | 0.3688 ± 0.0200 | 0.2808 ± 0.0489 | 0.6046 ± 0.0539 | 0.8351 ± 0.0290 | 0.1781 ± 0.0113 | 0.8463 ± 0.0120 |
| genRBF | 0.2443 ± 0.0019 | 0.6575 ± 0.0265 | 0.7345 ± 0.0280 | 0.4236 ± 0.0081 | 0.2059 ± 0.0036 | 0.1045 ± 0.0048 | 0.6202 ± 0.0387 | 0.7939 ± 0.0218 | 0.2195 ± 0.0429 | 0.8827 ± 0.0062 |
| KPCA | 0.2438 ± 0.0063 | 0.5161 ± 0.0213 | 0.8102 ± 0.0212 | 0.4707 ± 0.0507 | 0.3517 ± 0.0342 | 0.1817 ± 0.0052 | 0.7619 ± 0.0536 | 0.6500 ± 0.0467 | 0.2285 ± 0.0194 | 0.8610 ± 0.0110 |
| PPCA | 0.2384 ± 0.0032 | 0.4987 ± 0.0468 | 0.7702 ± 0.0215 | 0.4148 ± 0.0042 | 0.3339 ± 0.0200 | 0.1817 ± 0.0009 | 0.7142 ± 0.0579 | 0.5909 ± 0.0278 | 0.2281 ± 0.0183 | 0.7617 ± 0.0123 |
| HI- PMK | 0.2697 ± 0.0094 | 0.7500 ± 0.0358 | 0.7803 ± 0.0196 | 0.4605 ± 0.0516 | 0.4602 ± 0.0328 | 0.2694 ± 0.0443 | 0.7538 ± 0.0521 | 0.8673 ± 0.0112 | 0.2363 ± 0.0156 | 0.9329 ± 0.0064 |
| **MAR** | | | | | | | | | | |
| Mean | 0.2371 ± 0.0024 | 0.5115 ± 0.0419 | 0.8516 ± 0.0151 | 0.4781 ± 0.0007 | 0.5181 ± 0.0241 | 0.1848 ± 0.0009 | 0.7507 ± 0.0557 | 0.5755 ± 0.0197 | 0.2329 ± 0.0133 | 0.7780 ± 0.0137 |
| MICE | 0.2351 ± 0.0023 | 0.5245 ± 0.0400 | 0.8461 ± 0.0173 | 0.4715 ± 0.0007 | 0.5096 ± 0.0270 | 0.2159 ± 0.0009 | 0.7739 ± 0.0595 | 0.6347 ± 0.0243 | 0.2374 ± 0.0162 | 0.8515 ± 0.0131 |
| EM | 0.1960 ± 0.0059 | 0.4840 ± 0.0391 | 0.8255 ± 0.0227 | 0.4943 ± 0.0007 | 0.4560 ± 0.0276 | 0.2310 ± 0.0009 | 0.7117 ± 0.0516 | 0.5374 ± 0.0297 | 0.1792 ± 0.0156 | 0.7179 ± 0.0088 |
| MisF | 0.2710 ± 0.0071 | 0.7191 ± 0.0332 | 0.8550 ± 0.0131 | 0.4127 ± 0.0007 | 0.4626 ± 0.0299 | 0.2355 ± 0.0412 | 0.7556 ± 0.0588 | 0.5948 ± 0.0211 | 0.1706 ± 0.0287 | 0.9470 ± 0.0082 |
| GAIN | 0.2791 ± 0.0071 | 0.7905 ± 0.0278 | 0.8106 ± 0.0254 | 0.4133 ± 0.0018 | 0.4458 ± 0.0281 | 0.2814 ± 0.0504 | 0.6892 ± 0.0632 | 0.8665 ± 0.0385 | 0.1840 ± 0.0167 | 0.9077 ± 0.0125 |
| genRBF | NaN | 0.4543 ± 0.0368 | 0.8089 ± 0.0204 | 0.4667 ± 0.0007 | 0.4513 ± 0.0002 | 0.1889 ± 0.0009 | 0.6919 ± 0.0038 | 0.5002 ± 0.0131 | 0.1808 ± 0.0107 | 0.8235 ± 0.0074 |
| KPCA | 0.2084 ± 0.0093 | 0.4098 ± 0.0300 | 0.8707 ± 0.0154 | 0.5208 ± 0.0536 | 0.4264 ± 0.0330 | 0.2313 ± 0.0046 | 0.7819 ± 0.0557 | 0.6770 ± 0.0326 | 0.2402 ± 0.0174 | 0.8843 ± 0.0099 |
| PPCA | 0.2351 ± 0.0024 | 0.5236 ± 0.0396 | 0.8360 ± 0.0195 | 0.4526 ± 0.0305 | 0.4027 ± 0.0325 | 0.2270 ± 0.0009 | 0.7261 ± 0.0713 | 0.6229 ± 0.0246 | 0.2352 ± 0.0160 | 0.7857 ± 0.0142 |
| HI- PMK | 0.2852 ± 0.0071 | 0.7841 ± 0.0264 | 0.8390 ± 0.0193 | 0.5141 ± 0.0572 | 0.5250 ± 0.0285 | 0.2945 ± 0.0490 | 0.8129 ± 0.0658 | 0.8984 ± 0.0117 | 0.2429 ± 0.0115 | 0.9577 ± 0.0061 |
| **MNAR** | | | | | | | | | | |
| Model | Adult | Australian | Banknote | Breast | Car | Heart | Sonar | Spam | Student | Wine |
| Mean | 0.2129 ± 0.0026 | 0.6663 ± 0.0302 | 0.6855 ± 0.0186 | 0.4127 ± 0.0007 | 0.5025 ± 0.0298 | 0.1555 ± 0.0009 | 0.5402 ± 0.0427 | 0.7712 ± 0.0147 | 0.2072 ± 0.0313 | 0.7237 ± 0.0163 |
| MICE | 0.2316 ± 0.0026 | 0.6704 ± 0.0253 | 0.7034 ± 0.0222 | 0.4413 ± 0.0007 | 0.4950 ± 0.0298 | 0.2098 ± 0.0009 | 0.5809 ± 0.0451 | 0.7310 ± 0.0145 | 0.1757 ± 0.0351 | 0.7268 ± 0.0188 |
| EM | 0.2184 ± 0.0058 | 0.5538 ± 0.0294 | 0.7506 ± 0.0215 | 0.4746 ± 0.0007 | 0.3871 ± 0.0236 | 0.1547 ± 0.0009 | 0.5987 ± 0.0650 | 0.4988 ± 0.0211 | 0.1743 ± 0.0147 | 0.5309 ± 0.0072 |
| MisF | 0.2694 ± 0.0026 | 0.7200 ± 0.0318 | 0.7222 ± 0.0330 | 0.4638 ± 0.0400 | 0.3901 ± 0.0273 | 0.2672 ± 0.0429 | 0.6216 ± 0.0584 | 0.8913 ± 0.0202 | 0.1793 ± 0.0244 | 0.8658 ± 0.0110 |
| GAIN | 0.2769 ± 0.0026 | 0.7678 ± 0.0317 | 0.7710 ± 0.0614 | 0.4849 ± 0.0340 | 0.3117 ± 0.0264 | 0.2178 ± 0.0425 | 0.6414 ± 0.0660 | 0.8979 ± 0.0437 | 0.1806 ± 0.0155 | 0.8543 ± 0.0517 |
| genRBF | 0.1990 ± 0.0023 | 0.5967 ± 0.0380 | 0.6390 ± 0.0314 | 0.4719 ± 0.012 | 0.2059 ± 0.0002 | 0.2008 ± 0.0009 | 0.6973 ± 0.0543 | 0.8493 ± 0.0209 | 0.2050 ± 0.0097 | 0.8073 ± 0.0145 |
| KPCA | 0.1940 ± 0.0086 | 0.5967 ± 0.0291 | 0.8811 ± 0.0174 | 0.4919 ± 0.0641 | 0.4527 ± 0.0393 | 0.1882 ± 0.0111 | 0.7471 ± 0.0518 | 0.7516 ± 0.0267 | 0.2275 ± 0.0147 | 0.8034 ± 0.0222 |
| PPCA | 0.2311 ± 0.0026 | 0.5791 ± 0.0271 | 0.7915 ± 0.0404 | 0.4541 ± 0.0007 | 0.3885 ± 0.0311 | 0.1870 ± 0.0009 | 0.5289 ± 0.0391 | 0.5493 ± 0.0289 | 0.2181 ± 0.0158 | 0.8483 ± 0.0126 |
| HI- PMK | 0.2858 ± 0.0104 | 0.7851 ± 0.0332 | 0.8253 ± 0.0256 | 0.4925 ± 0.0400 | 0.5030 ± 0.0312 | 0.2825 ± 0.0520 | 0.7737 ± 0.0358 | 0.9347 ± 0.0109 | 0.2290 ± 0.0099 | 0.9111± 0.01475 |

Table 6: Average F1 scores with standard deviations for classification tasks on complete datasets.

| Type | Model | 0.05 | 0.1 | 0.2 | 0.3 | 0.4 | 0.5 | 0.6 | 0.7 | 0.8 |
|---|---|---|---|---|---|---|---|---|---|---|
| MCAR | Mean | 0.6590 ± 0.040 | 0.6528 ± 0.027 | 0.6408 ± 0.035 | 0.6428 ± 0.043 | 0.6287 ± 0.026 | 0.6103 ± 0.036 | 0.5999 ± 0.043 | 0.5679 ± 0.059 | 0.5118 ± 0.046 |
| | MICE | 0.6532 ± 0.033 | 0.6568 ± 0.033 | 0.6239 ± 0.038 | 0.6390 ± 0.041 | 0.6066 ± 0.047 | 0.6559 ± 0.038 | 0.5226 ± 0.035 | 0.5879 ± 0.047 | 0.5647 ± 0.047 |
| | EM | 0.5818 ± 0.019 | 0.5586 ± 0.027 | 0.5408 ± 0.051 | 0.5286 ± 0.035 | 0.4545 ± 0.063 | 0.4201 ± 0.073 | 0.4448 ± 0.061 | 0.4071 ± 0.042 | 0.3833 ± 0.040 |
| | MisF | 0.8447 ± 0.014 | 0.8253 ± 0.029 | 0.7839 ± 0.023 | 0.7458 ± 0.023 | 0.7153 ± 0.029 | 0.6731 ± 0.034 | 0.5765 ± 0.026 | 0.5407 ± 0.025 | 0.5128 ± 0.054 |
| | GAIN | 0.8252 ± 0.025 | 0.8233 ± 0.020 | 0.8086 ± 0.019 | 0.7780 ± 0.025 | 0.7795 ± 0.013 | 0.7563 ± 0.026 | 0.7179 ± 0.026 | 0.6749 ± 0.045 | 0.6287 ± 0.032 |
| | genRBF | 0.8541 ± 0.030 | 0.8451 ± 0.030 | 0.8269 ± 0.018 | 0.7714 ± 0.022 | 0.7014 ± 0.029 | 0.6155 ± 0.032 | 0.5002 ± 0.036 | 0.4216 ± 0.024 | 0.3812 ± 0.019 |
| | KPCA | 0.5887 ± 0.008 | 0.5704 ± 0.014 | 0.5452 ± 0.019 | 0.5376 ± 0.006 | 0.5195 ± 0.017 | 0.5184 ± 0.034 | 0.4741 ± 0.007 | 0.4681 ± 0.046 | 0.4227 ± 0.042 |
| | PPCA | 0.5764 ± 0.021 | 0.5631 ± 0.023 | 0.5424 ± 0.068 | 0.5356 ± 0.043 | 0.4645 ± 0.039 | 0.4759 ± 0.103 | 0.5138 ± 0.054 | 0.4198 ± 0.036 | 0.3968 ± 0.035 |
| | HI- PMK | 0.8231 ± 0.031 | 0.8166 ± 0.033 | 0.8061 ± 0.039 | 0.7928 ± 0.043 | 0.7741 ± 0.039 | 0.7668 ± 0.040 | 0.7125 ± 0.028 | 0.6554 ± 0.045 | 0.6029 ± 0.025 |
| MAR | Mean | 0.5711 ± 0.033 | 0.5961 ± 0.030 | 0.5404 ± 0.035 | 0.5008 ± 0.022 | 0.5457 ± 0.082 | 0.4754 ± 0.055 | 0.4836 ± 0.054 | 0.4198 ± 0.029 | 0.4706 ± 0.037 |
| | MICE | 0.5685 ± 0.026 | 0.5744 ± 0.039 | 0.5553 ± 0.027 | 0.5018 ± 0.022 | 0.5588 ± 0.057 | 0.6335 ± 0.037 | 0.4395 ± 0.051 | 0.4492 ± 0.065 | 0.4392 ± 0.035 |
| | EM | 0.5765 ± 0.021 | 0.5761 ± 0.025 | 0.5278 ± 0.037 | 0.4494 ± 0.053 | 0.5962 ± 0.017 | 0.4000 ± 0.059 | 0.4588 ± 0.079 | 0.3783 ± 0.025 | 0.3928 ± 0.037 |
| | MisF | 0.8416 ± 0.026 | 0.8276 ± 0.028 | 0.8204 ± 0.020 | 0.8198 ± 0.009 | 0.7756 ± 0.036 | 0.6545 ± 0.032 | 0.6423 ± 0.062 | 0.5332 ± 0.018 | 0.5568 ± 0.069 |
| | GAIN | 0.8305 ± 0.025 | 0.8342 ± 0.019 | 0.8246 ± 0.017 | 0.8490 ± 0.008 | 0.7868 ± 0.023 | 0.7597 ± 0.039 | 0.7649 ± 0.042 | 0.7348 ± 0.030 | 0.7299 ± 0.046 |
| | genRBF | 0.4859 ± 0.042 | 0.4895 ± 0.040 | 0.4688 ± 0.028 | 0.4767 ± 0.036 | 0.4576 ± 0.056 | 0.4611 ± 0.044 | 0.4039 ± 0.023 | 0.4483 ± 0.033 | 0.3970 ± 0.029 |
| | KPCA | 0.3631 ± 0.009 | 0.3646 ± 0.006 | 0.3597 ± 0.010 | 0.3726 ± 0.011 | 0.3539 ± 0.003 | 0.3612 ± 0.011 | 0.4018 ± 0.047 | 0.6086 ± 0.070 | 0.5028 ± 0.103 |
| | PPCA | 0.5674 ± 0.026 | 0.5755 ± 0.038 | 0.5553 ± 0.027 | 0.5018 ± 0.022 | 0.5598 ± 0.057 | 0.6310 ± 0.039 | 0.4382 ± 0.048 | 0.4471 ± 0.061 | 0.4361 ± 0.037 |
| | HI- PMK | 0.8355 ± 0.019 | 0.8164 ± 0.024 | 0.8052 ± 0.026 | 0.8048 ± 0.010 | 0.7915 ± 0.026 | 0.7738 ± 0.024 | 0.7697 ± 0.048 | 0.7198 ± 0.019 | 0.7399 ± 0.041 |
| MNAR | Mean | 0.6684 ± 0.021 | 0.6639 ± 0.018 | 0.6496 ± 0.026 | 0.6842 ± 0.015 | 0.6959 ± 0.033 | 0.6952 ± 0.036 | 0.6509 ± 0.049 | 0.6653 ± 0.036 | 0.6236 ± 0.038 |
| | MICE | 0.6642 ± 0.023 | 0.6697 ± 0.020 | 0.6780 ± 0.041 | 0.6914 ± 0.012 | 0.7060 ± 0.032 | 0.6639 ± 0.014 | 0.6257 ± 0.015 | 0.6545 ± 0.048 | 0.6803 ± 0.024 |
| | EM | 0.5962 ± 0.017 | 0.5962 ± 0.017 | 0.5962 ± 0.017 | 0.5962 ± 0.017 | 0.5962 ± 0.017 | 0.5014 ± 0.051 | 0.4925 ± 0.030 | 0.5006 ± 0.040 | 0.5086 ± 0.059 |
| | MisF | 0.8524 ± 0.015 | 0.8482 ± 0.022 | 0.8278 ± 0.023 | 0.7326 ± 0.033 | 0.7370 ± 0.016 | 0.7110 ± 0.040 | 0.6299 ± 0.044 | 0.5772 ± 0.043 | 0.5636 ± 0.050 |
| | GAIN | 0.8292 ± 0.030 | 0.8347 ± 0.022 | 0.8237 ± 0.030 | 0.8149 ± 0.021 | 0.7741 ± 0.035 | 0.7460 ± 0.038 | 0.7199 ± 0.029 | 0.6719 ± 0.030 | 0.6955 ± 0.050 |
| | genRBF | 0.5962 ± 0.043 | 0.5962 ± 0.039 | 0.5962 ± 0.032 | 0.5962 ± 0.031 | 0.5962 ± 0.018 | 0.5962 ± 0.079 | 0.5983 ± 0.017 | 0.6003 ± 0.024 | 0.5940 ± 0.024 |
| | KPCA | 0.5962 ± 0.010 | 0.5962 ± 0.012 | 0.5962 ± 0.013 | 0.5962 ± 0.013 | 0.5962 ± 0.018 | 0.5962 ± 0.013 | 0.5983 ± 0.005 | 0.6003 ± 0.133 | 0.5940 ± 0.045 |
| | PPCA | 0.5962 ± 0.017 | 0.5962 ± 0.017 | 0.5962 ± 0.017 | 0.5983 ± 0.020 | 0.5983 ± 0.020 | 0.5676 ± 0.018 | 0.5240 ± 0.035 | 0.5578 ± 0.087 | 0.5777 ± 0.012 |
| | HI- PMK | 0.8357 ± 0.012 | 0.8214 ± 0.016 | 0.8149 ± 0.033 | 0.8082 ± 0.039 | 0.7863 ± 0.056 | 0.7785 ± 0.046 | 0.7696 ± 0.040 | 0.7349 ± 0.027 | 0.7166 ± 0.029 |

Table 7: Detailed F1 scores and standard deviation for the **Australian** dataset.

| Type | Model | 0.05 | 0.1 | 0.2 | 0.3 | 0.4 | 0.5 | 0.6 | 0.7 | 0.8 |
|---|---|---|---|---|---|---|---|---|---|---|
| MCAR | Mean | 0.9475 ± 0.006 | 0.9201 ± 0.009 | 0.8791 ± 0.007 | 0.8376 ± 0.012 | 0.7824 ± 0.011 | 0.7309 ± 0.015 | 0.6679 ± 0.037 | 0.6007 ± 0.047 | 0.4905 ± 0.041 |
| | MICE | 0.9660 ± 0.007 | 0.9444 ± 0.010 | 0.9014 ± 0.005 | 0.8532 ± 0.005 | 0.8041 ± 0.007 | 0.7350 ± 0.010 | 0.6445 ± 0.034 | 0.5782 ± 0.037 | 0.5256 ± 0.032 |
| | EM | 0.9631 ± 0.003 | 0.9262 ± 0.016 | 0.8582 ± 0.031 | 0.8223 ± 0.020 | 0.7798 ± 0.013 | 0.7407 ± 0.027 | 0.6848 ± 0.024 | 0.6099 ± 0.019 | 0.5529 ± 0.041 |
| | MisF | 0.9831 ± 0.008 | 0.9684 ± 0.012 | 0.9323 ± 0.015 | 0.8918 ± 0.017 | 0.8428 ± 0.018 | 0.7807 ± 0.015 | 0.7019 ± 0.012 | 0.6354 ± 0.022 | 0.5617 ± 0.023 |
| | GAIN | 0.9461 ± 0.026 | 0.9246 ± 0.008 | 0.8635 ± 0.029 | 0.8130 ± 0.019 | 0.7747 ± 0.025 | 0.7255 ± 0.023 | 0.6645 ± 0.026 | 0.5980 ± 0.025 | 0.5417 ± 0.026 |
| | genRBF | 0.9416 ± 0.004 | 0.9156 ± 0.008 | 0.8679 ± 0.010 | 0.8143 ± 0.015 | 0.7445 ± 0.034 | 0.6893 ± 0.030 | 0.6350 ± 0.047 | 0.5563 ± 0.042 | 0.4455 ± 0.062 |
| | KPCA | 0.9830 ± 0.008 | 0.9609 ± 0.006 | 0.9298 ± 0.020 | 0.8873 ± 0.019 | 0.8203 ± 0.037 | 0.7666 ± 0.031 | 0.7090 ± 0.013 | 0.6495 ± 0.017 | 0.5851 ± 0.039 |
| | PPCA | 0.9547 ± 0.020 | 0.9422 ± 0.012 | 0.8957 ± 0.017 | 0.8410 ± 0.014 | 0.7944 ± 0.022 | 0.7243 ± 0.020 | 0.6524 ± 0.015 | 0.5777 ± 0.034 | 0.5494 ± 0.040 |
| | HI- PMK | 0.9683 ± 0.011 | 0.9411 ± 0.021 | 0.8885 ± 0.023 | 0.8377 ± 0.010 | 0.7883 ± 0.023 | 0.7194 ± 0.021 | 0.6680 ± 0.015 | 0.6472 ± 0.015 | 0.5641 ± 0.038 |
| MAR | Mean | 0.9794 ± 0.006 | 0.9521 ± 0.010 | 0.9610 ± 0.007 | 0.8914 ± 0.015 | 0.9124 ± 0.008 | 0.7725 ± 0.029 | 0.9012 ± 0.014 | 0.7258 ± 0.033 | 0.5683 ± 0.014 |
| | MICE | 0.9779 ± 0.006 | 0.9490 ± 0.014 | 0.9601 ± 0.010 | 0.9265 ± 0.014 | 0.9126 ± 0.011 | 0.7562 ± 0.026 | 0.8881 ± 0.011 | 0.6953 ± 0.037 | 0.5488 ± 0.027 |
| | EM | 0.9757 ± 0.007 | 0.9322 ± 0.011 | 0.9499 ± 0.019 | 0.8664 ± 0.018 | 0.8701 ± 0.017 | 0.7382 ± 0.038 | 0.8737 ± 0.024 | 0.6717 ± 0.033 | 0.5514 ± 0.036 |
| | MisF | 0.9853 ± 0.005 | 0.9698 ± 0.008 | 0.9610 ± 0.009 | 0.8983 ± 0.015 | 0.9182 ± 0.006 | 0.7899 ± 0.014 | 0.8951 ± 0.021 | 0.6979 ± 0.014 | 0.5793 ± 0.025 |
| | GAIN | 0.9565 ± 0.010 | 0.9242 ± 0.019 | 0.9269 ± 0.003 | 0.8537 ± 0.042 | 0.8740 ± 0.032 | 0.7284 ± 0.036 | 0.8713 ± 0.037 | 0.6415 ± 0.030 | 0.5189 ± 0.019 |
| | genRBF | 0.9558 ± 0.018 | 0.9038 ± 0.014 | 0.9061 ± 0.033 | 0.8532 ± 0.021 | 0.8237 ± 0.019 | 0.7255 ± 0.022 | 0.7550 ± 0.019 | 0.7015 ± 0.015 | 0.6553 ± 0.021 |
| | KPCA | 0.9897 ± 0.004 | 0.9756 ± 0.008 | 0.9749 ± 0.016 | 0.9377 ± 0.007 | 0.9360 ± 0.014 | 0.7751 ± 0.025 | 0.8952 ± 0.013 | 0.7320 ± 0.028 | 0.6201 ± 0.024 |
| | PPCA | 0.9779 ± 0.006 | 0.9369 ± 0.023 | 0.9504 ± 0.014 | 0.9243 ± 0.016 | 0.9052 ± 0.015 | 0.7015 ± 0.027 | 0.8850 ± 0.009 | 0.6941 ± 0.037 | 0.5491 ± 0.028 |
| | HI- PMK | 0.9698 ± 0.008 | 0.9454 ± 0.016 | 0.9470 ± 0.009 | 0.9182 ± 0.010 | 0.8813 ± 0.014 | 0.7381 ± 0.029 | 0.8795 ± 0.011 | 0.6997 ± 0.033 | 0.5722 ± 0.043 |
| MNAR | Mean | 0.8848 ± 0.018 | 0.8724 ± 0.016 | 0.8335 ± 0.012 | 0.7877 ± 0.014 | 0.7193 ± 0.011 | 0.6606 ± 0.021 | 0.5758 ± 0.031 | 0.4390 ± 0.024 | 0.3962 ± 0.020 |
| | MICE | 0.9112 ± 0.013 | 0.8846 ± 0.017 | 0.8564 ± 0.022 | 0.8353 ± 0.025 | 0.7036 ± 0.022 | 0.6575 ± 0.015 | 0.5809 ± 0.028 | 0.4635 ± 0.026 | 0.4376 ± 0.030 |
| | EM | 0.9471 ± 0.016 | 0.9233 ± 0.013 | 0.8804 ± 0.017 | 0.8179 ± 0.026 | 0.7663 ± 0.016 | 0.7059 ± 0.005 | 0.6762 ± 0.035 | 0.5362 ± 0.040 | 0.5025 ± 0.025 |
| | MisF | 0.8804 ± 0.020 | 0.8409 ± 0.013 | 0.8373 ± 0.012 | 0.8049 ± 0.012 | 0.7410 ± 0.027 | 0.7022 ± 0.019 | 0.6330 ± 0.058 | 0.6030 ± 0.118 | 0.4573 ± 0.018 |
| | GAIN | 0.9141 ± 0.029 | 0.8831 ± 0.048 | 0.8371 ± 0.012 | 0.8529 ± 0.023 | 0.7835 ± 0.036 | 0.6933 ± 0.064 | 0.7379 ± 0.079 | 0.6331 ± 0.155 | 0.6037 ± 0.107 |
| | genRBF | 0.8439 ± 0.019 | 0.7860 ± 0.018 | 0.7967 ± 0.018 | 0.7562 ± 0.035 | 0.6606 ± 0.045 | 0.6242 ± 0.039 | 0.5099 ± 0.065 | 0.3990 ± 0.025 | 0.3745 ± 0.018 |
| | KPCA | 0.9941 ± 0.006 | 0.9882 ± 0.006 | 0.9757 ± 0.009 | 0.9331 ± 0.013 | 0.8963 ± 0.019 | 0.7990 ± 0.034 | 0.8202 ± 0.029 | 0.7879 ± 0.017 | 0.7357 ± 0.023 |
| | PPCA | 0.9614 ± 0.016 | 0.9533 ± 0.014 | 0.9081 ± 0.027 | 0.8516 ± 0.014 | 0.8025 ± 0.019 | 0.6838 ± 0.023 | 0.7268 ± 0.034 | 0.6486 ± 0.115 | 0.5873 ± 0.101 |
| | HI- PMK | 0.9322 ± 0.019 | 0.9183 ± 0.015 | 0.8760 ± 0.015 | 0.8357 ± 0.019 | 0.8118 ± 0.017 | 0.7233 ± 0.025 | 0.7865 ± 0.039 | 0.7981 ± 0.048 | 0.7458 ± 0.035 |

Table 8: Detailed F1 scores and standard deviation for the **Banknote** dataset.

| Type | Model | 0.05 | 0.1 | 0.2 | 0.3 | 0.4 | 0.5 | 0.6 | 0.7 | 0.8 |
|---|---|---|---|---|---|---|---|---|---|---|
| MCAR | Mean | 0.9475 ± 0.006 | 0.9201 ± 0.009 | 0.8791 ± 0.007 | 0.8376 ± 0.012 | 0.7824 ± 0.011 | 0.7309 ± 0.015 | 0.6679 ± 0.037 | 0.6007 ± 0.047 | 0.4905 ± 0.041 |
| | MICE | 0.9660 ± 0.007 | 0.9444 ± 0.010 | 0.9014 ± 0.005 | 0.8532 ± 0.005 | 0.8041 ± 0.007 | 0.7350 ± 0.010 | 0.6445 ± 0.034 | 0.5782 ± 0.037 | 0.5256 ± 0.032 |
| | EM | 0.9631 ± 0.003 | 0.9262 ± 0.016 | 0.8582 ± 0.031 | 0.8223 ± 0.020 | 0.7798 ± 0.013 | 0.7407 ± 0.027 | 0.6848 ± 0.024 | 0.6099 ± 0.019 | 0.5529 ± 0.041 |
| | MisF | 0.9831 ± 0.008 | 0.9684 ± 0.012 | 0.9323 ± 0.015 | 0.8918 ± 0.017 | 0.8428 ± 0.018 | 0.7807 ± 0.015 | 0.7019 ± 0.012 | 0.6354 ± 0.022 | 0.5617 ± 0.023 |
| | GAIN | 0.9461 ± 0.026 | 0.9246 ± 0.008 | 0.8635 ± 0.029 | 0.8130 ± 0.019 | 0.7747 ± 0.025 | 0.7255 ± 0.023 | 0.6645 ± 0.026 | 0.5980 ± 0.025 | 0.5417 ± 0.026 |
| | genRBF | 0.9416 ± 0.004 | 0.9156 ± 0.008 | 0.8679 ± 0.010 | 0.8143 ± 0.015 | 0.7445 ± 0.034 | 0.6893 ± 0.030 | 0.6350 ± 0.047 | 0.5563 ± 0.042 | 0.4455 ± 0.062 |
| | KPCA | 0.9830 ± 0.008 | 0.9609 ± 0.006 | 0.9298 ± 0.020 | 0.8873 ± 0.019 | 0.8203 ± 0.037 | 0.7666 ± 0.031 | 0.7090 ± 0.013 | 0.6495 ± 0.017 | 0.5851 ± 0.039 |
| | PPCA | 0.9547 ± 0.020 | 0.9422 ± 0.012 | 0.8957 ± 0.017 | 0.8410 ± 0.014 | 0.7944 ± 0.022 | 0.7243 ± 0.020 | 0.6524 ± 0.015 | 0.5777 ± 0.034 | 0.5494 ± 0.040 |
| | HI- PMK | 0.9683 ± 0.011 | 0.9411 ± 0.021 | 0.8885 ± 0.023 | 0.8377 ± 0.010 | 0.7883 ± 0.023 | 0.7194 ± 0.021 | 0.6680 ± 0.015 | 0.6472 ± 0.015 | 0.5641 ± 0.038 |
| MAR | Mean | 0.9794 ± 0.006 | 0.9521 ± 0.010 | 0.9610 ± 0.007 | 0.8914 ± 0.015 | 0.9124 ± 0.008 | 0.7725 ± 0.029 | 0.9012 ± 0.014 | 0.7258 ± 0.033 | 0.5683 ± 0.014 |
| | MICE | 0.9779 ± 0.006 | 0.9490 ± 0.014 | 0.9601 ± 0.010 | 0.9265 ± 0.014 | 0.9126 ± 0.011 | 0.7562 ± 0.026 | 0.8881 ± 0.011 | 0.6953 ± 0.037 | 0.5488 ± 0.027 |
| | EM | 0.9757 ± 0.007 | 0.9322 ± 0.011 | 0.9499 ± 0.019 | 0.8664 ± 0.018 | 0.8701 ± 0.017 | 0.7382 ± 0.038 | 0.8737 ± 0.024 | 0.6717 ± 0.033 | 0.5514 ± 0.036 |
| | MisF | 0.9853 ± 0.005 | 0.9698 ± 0.008 | 0.9610 ± 0.009 | 0.8983 ± 0.015 | 0.9182 ± 0.006 | 0.7899 ± 0.014 | 0.8951 ± 0.021 | 0.6979 ± 0.014 | 0.5793 ± 0.025 |
| | GAIN | 0.9565 ± 0.010 | 0.9242 ± 0.019 | 0.9269 ± 0.003 | 0.8537 ± 0.042 | 0.8740 ± 0.032 | 0.7284 ± 0.036 | 0.8713 ± 0.037 | 0.6415 ± 0.030 | 0.5189 ± 0.019 |
| | genRBF | 0.9558 ± 0.018 | 0.9038 ± 0.014 | 0.9061 ± 0.033 | 0.8532 ± 0.021 | 0.8237 ± 0.019 | 0.7255 ± 0.022 | 0.7550 ± 0.019 | 0.7015 ± 0.015 | 0.6553 ± 0.021 |
| | KPCA | 0.9897 ± 0.004 | 0.9756 ± 0.008 | 0.9749 ± 0.016 | 0.9377 ± 0.007 | 0.9360 ± 0.014 | 0.7751 ± 0.025 | 0.8952 ± 0.013 | 0.7320 ± 0.028 | 0.6201 ± 0.024 |
| | PPCA | 0.9779 ± 0.006 | 0.9369 ± 0.023 | 0.9504 ± 0.014 | 0.9243 ± 0.016 | 0.9052 ± 0.015 | 0.7015 ± 0.027 | 0.8850 ± 0.009 | 0.6941 ± 0.037 | 0.5491 ± 0.028 |
| | HI- PMK | 0.9698 ± 0.008 | 0.9454 ± 0.016 | 0.9470 ± 0.009 | 0.9182 ± 0.010 | 0.8813 ± 0.014 | 0.7381 ± 0.029 | 0.8795 ± 0.011 | 0.6997 ± 0.033 | 0.5722 ± 0.043 |
| MNAR | Mean | 0.8848 ± 0.018 | 0.8724 ± 0.016 | 0.8335 ± 0.012 | 0.7877 ± 0.014 | 0.7193 ± 0.011 | 0.6606 ± 0.021 | 0.5758 ± 0.031 | 0.4390 ± 0.024 | 0.3962 ± 0.020 |
| | MICE | 0.9112 ± 0.013 | 0.8846 ± 0.017 | 0.8564 ± 0.022 | 0.8353 ± 0.025 | 0.7036 ± 0.022 | 0.6575 ± 0.015 | 0.5809 ± 0.028 | 0.4635 ± 0.026 | 0.4376 ± 0.030 |
| | EM | 0.9471 ± 0.016 | 0.9233 ± 0.013 | 0.8804 ± 0.017 | 0.8179 ± 0.026 | 0.7663 ± 0.016 | 0.7059 ± 0.005 | 0.6762 ± 0.035 | 0.5362 ± 0.040 | 0.5025 ± 0.025 |
| | MisF | 0.8804 ± 0.020 | 0.8409 ± 0.013 | 0.8373 ± 0.012 | 0.8049 ± 0.012 | 0.7410 ± 0.027 | 0.7022 ± 0.019 | 0.6330 ± 0.058 | 0.6030 ± 0.118 | 0.4573 ± 0.018 |
| | GAIN | 0.9141 ± 0.029 | 0.8831 ± 0.048 | 0.8371 ± 0.012 | 0.8529 ± 0.023 | 0.7835 ± 0.036 | 0.6933 ± 0.064 | 0.7379 ± 0.079 | 0.6331 ± 0.155 | 0.6037 ± 0.107 |
| | genRBF | 0.8439 ± 0.019 | 0.7860 ± 0.018 | 0.7967 ± 0.018 | 0.7562 ± 0.035 | 0.6606 ± 0.045 | 0.6242 ± 0.039 | 0.5099 ± 0.065 | 0.3990 ± 0.025 | 0.3745 ± 0.018 |
| | KPCA | 0.9941 ± 0.006 | 0.9882 ± 0.006 | 0.9757 ± 0.009 | 0.9331 ± 0.013 | 0.8963 ± 0.019 | 0.7990 ± 0.034 | 0.8202 ± 0.029 | 0.7879 ± 0.017 | 0.7357 ± 0.023 |
| | PPCA | 0.9614 ± 0.016 | 0.9533 ± 0.014 | 0.9081 ± 0.027 | 0.8516 ± 0.014 | 0.8025 ± 0.019 | 0.6838 ± 0.023 | 0.7268 ± 0.034 | 0.6486 ± 0.115 | 0.5873 ± 0.101 |
| | HI- PMK | 0.9322 ± 0.019 | 0.9183 ± 0.015 | 0.8760 ± 0.015 | 0.8357 ± 0.019 | 0.8118 ± 0.017 | 0.7233 ± 0.025 | 0.7865 ± 0.039 | 0.7981 ± 0.048 | 0.7458 ± 0.035 |

Table 9: Detailed F1 scores and standard deviation for the **Breast** dataset.

| Type | Model | 0.05 | 0.1 | 0.2 | 0.3 | 0.4 | 0.5 | 0.6 | 0.7 | 0.8 |
|---|---|---|---|---|---|---|---|---|---|---|
| MCAR | Mean | 0.9475 ± 0.006 | 0.9201 ± 0.009 | 0.8791 ± 0.007 | 0.8376 ± 0.012 | 0.7824 ± 0.011 | 0.7309 ± 0.015 | 0.6679 ± 0.037 | 0.6007 ± 0.047 | 0.4905 ± 0.041 |
| | MICE | 0.9660 ± 0.007 | 0.9444 ± 0.010 | 0.9014 ± 0.005 | 0.8532 ± 0.005 | 0.8041 ± 0.007 | 0.7350 ± 0.010 | 0.6445 ± 0.034 | 0.5782 ± 0.037 | 0.5256 ± 0.032 |
| | EM | 0.9631 ± 0.003 | 0.9262 ± 0.016 | 0.8582 ± 0.031 | 0.8223 ± 0.020 | 0.7798 ± 0.013 | 0.7407 ± 0.027 | 0.6848 ± 0.024 | 0.6099 ± 0.019 | 0.5529 ± 0.041 |
| | MisF | 0.9831 ± 0.008 | 0.9684 ± 0.012 | 0.9323 ± 0.015 | 0.8918 ± 0.017 | 0.8428 ± 0.018 | 0.7807 ± 0.015 | 0.7019 ± 0.012 | 0.6354 ± 0.022 | 0.5617 ± 0.023 |
| | GAIN | 0.9461 ± 0.026 | 0.9246 ± 0.008 | 0.8635 ± 0.029 | 0.8130 ± 0.019 | 0.7747 ± 0.025 | 0.7255 ± 0.023 | 0.6645 ± 0.026 | 0.5980 ± 0.025 | 0.5417 ± 0.026 |
| | genRBF | 0.9416 ± 0.004 | 0.9156 ± 0.008 | 0.8679 ± 0.010 | 0.8143 ± 0.015 | 0.7445 ± 0.034 | 0.6893 ± 0.030 | 0.6350 ± 0.047 | 0.5563 ± 0.042 | 0.4455 ± 0.062 |
| | KPCA | 0.9830 ± 0.008 | 0.9609 ± 0.006 | 0.9298 ± 0.020 | 0.8873 ± 0.019 | 0.8203 ± 0.037 | 0.7666 ± 0.031 | 0.7090 ± 0.013 | 0.6495 ± 0.017 | 0.5851 ± 0.039 |
| | PPCA | 0.9547 ± 0.020 | 0.9422 ± 0.012 | 0.8957 ± 0.017 | 0.8410 ± 0.014 | 0.7944 ± 0.022 | 0.7243 ± 0.020 | 0.6524 ± 0.015 | 0.5777 ± 0.034 | 0.5494 ± 0.040 |
| | HI- PMK | 0.9683 ± 0.011 | 0.9411 ± 0.021 | 0.8885 ± 0.023 | 0.8377 ± 0.010 | 0.7883 ± 0.023 | 0.7194 ± 0.021 | 0.6680 ± 0.015 | 0.6472 ± 0.015 | 0.5641 ± 0.038 |
| MAR | Mean | 0.9794 ± 0.006 | 0.9521 ± 0.010 | 0.9610 ± 0.007 | 0.8914 ± 0.015 | 0.9124 ± 0.008 | 0.7725 ± 0.029 | 0.9012 ± 0.014 | 0.7258 ± 0.033 | 0.5683 ± 0.014 |
| | MICE | 0.9779 ± 0.006 | 0.9490 ± 0.014 | 0.9601 ± 0.010 | 0.9265 ± 0.014 | 0.9126 ± 0.011 | 0.7562 ± 0.026 | 0.8881 ± 0.011 | 0.6953 ± 0.037 | 0.5488 ± 0.027 |
| | EM | 0.9757 ± 0.007 | 0.9322 ± 0.011 | 0.9499 ± 0.019 | 0.8664 ± 0.018 | 0.8701 ± 0.017 | 0.7382 ± 0.038 | 0.8737 ± 0.024 | 0.6717 ± 0.033 | 0.5514 ± 0.036 |
| | MisF | 0.9853 ± 0.005 | 0.9698 ± 0.008 | 0.9610 ± 0.009 | 0.8983 ± 0.015 | 0.9182 ± 0.006 | 0.7899 ± 0.014 | 0.8951 ± 0.021 | 0.6979 ± 0.014 | 0.5793 ± 0.025 |
| | GAIN | 0.9565 ± 0.010 | 0.9242 ± 0.019 | 0.9269 ± 0.003 | 0.8537 ± 0.042 | 0.8740 ± 0.032 | 0.7284 ± 0.036 | 0.8713 ± 0.037 | 0.6415 ± 0.030 | 0.5189 ± 0.019 |
| | genRBF | 0.9558 ± 0.018 | 0.9038 ± 0.014 | 0.9061 ± 0.033 | 0.8532 ± 0.021 | 0.8237 ± 0.019 | 0.7255 ± 0.022 | 0.7550 ± 0.019 | 0.7015 ± 0.015 | 0.6553 ± 0.021 |
| | KPCA | 0.9897 ± 0.004 | 0.9756 ± 0.008 | 0.9749 ± 0.016 | 0.9377 ± 0.007 | 0.9360 ± 0.014 | 0.7751 ± 0.025 | 0.8952 ± 0.013 | 0.7320 ± 0.028 | 0.6201 ± 0.024 |
| | PPCA | 0.9779 ± 0.006 | 0.9369 ± 0.023 | 0.9504 ± 0.014 | 0.9243 ± 0.016 | 0.9052 ± 0.015 | 0.7015 ± 0.027 | 0.8850 ± 0.009 | 0.6941 ± 0.037 | 0.5491 ± 0.028 |
| | HI- PMK | 0.9698 ± 0.008 | 0.9454 ± 0.016 | 0.9470 ± 0.009 | 0.9182 ± 0.010 | 0.8813 ± 0.014 | 0.7381 ± 0.029 | 0.8795 ± 0.011 | 0.6997 ± 0.033 | 0.5722 ± 0.043 |
| MNAR | Mean | 0.8848 ± 0.018 | 0.8724 ± 0.016 | 0.8335 ± 0.012 | 0.7877 ± 0.014 | 0.7193 ± 0.011 | 0.6606 ± 0.021 | 0.5758 ± 0.031 | 0.4390 ± 0.024 | 0.3962 ± 0.020 |
| | MICE | 0.9112 ± 0.013 | 0.8846 ± 0.017 | 0.8564 ± 0.022 | 0.8353 ± 0.025 | 0.7036 ± 0.022 | 0.6575 ± 0.015 | 0.5809 ± 0.028 | 0.4635 ± 0.026 | 0.4376 ± 0.030 |
| | EM | 0.9471 ± 0.016 | 0.9233 ± 0.013 | 0.8804 ± 0.017 | 0.8179 ± 0.026 | 0.7663 ± 0.016 | 0.7059 ± 0.005 | 0.6762 ± 0.035 | 0.5362 ± 0.040 | 0.5025 ± 0.025 |
| | MisF | 0.8804 ± 0.020 | 0.8409 ± 0.013 | 0.8373 ± 0.012 | 0.8049 ± 0.012 | 0.7410 ± 0.027 | 0.7022 ± 0.019 | 0.6330 ± 0.058 | 0.6030 ± 0.118 | 0.4573 ± 0.018 |
| | GAIN | 0.9141 ± 0.029 | 0.8831 ± 0.048 | 0.8371 ± 0.012 | 0.8529 ± 0.023 | 0.7835 ± 0.036 | 0.6933 ± 0.064 | 0.7379 ± 0.079 | 0.6331 ± 0.155 | 0.6037 ± 0.107 |
| | genRBF | 0.8439 ± 0.019 | 0.7860 ± 0.018 | 0.7967 ± 0.018 | 0.7562 ± 0.035 | 0.6606 ± 0.045 | 0.6242 ± 0.039 | 0.5099 ± 0.065 | 0.3990 ± 0.025 | 0.3745 ± 0.018 |
| | KPCA | 0.9941 ± 0.006 | 0.9882 ± 0.006 | 0.9757 ± 0.009 | 0.9331 ± 0.013 | 0.8963 ± 0.019 | 0.7990 ± 0.034 | 0.8202 ± 0.029 | 0.7879 ± 0.017 | 0.7357 ± 0.023 |
| | PPCA | 0.9614 ± 0.016 | 0.9533 ± 0.014 | 0.9081 ± 0.027 | 0.8516 ± 0.014 | 0.8025 ± 0.019 | 0.6838 ± 0.023 | 0.7268 ± 0.034 | 0.6486 ± 0.115 | 0.5873 ± 0.101 |
| | HI- PMK | 0.9322 ± 0.019 | 0.9183 ± 0.015 | 0.8760 ± 0.015 | 0.8357 ± 0.019 | 0.8118 ± 0.017 | 0.7233 ± 0.025 | 0.7865 ± 0.039 | 0.7981 ± 0.048 | 0.7458 ± 0.035 |

Table 10: Detailed F1 scores and standard deviation for the **Car** dataset.

| Type | Model | 0.05 | 0.1 | 0.2 | 0.3 | 0.4 | 0.5 | 0.6 | 0.7 | 0.8 |
|---|---|---|---|---|---|---|---|---|---|---|
| MCAR | Mean | 0.9475 ± 0.006 | 0.9201 ± 0.009 | 0.8791 ± 0.007 | 0.8376 ± 0.012 | 0.7824 ± 0.011 | 0.7309 ± 0.015 | 0.6679 ± 0.037 | 0.6007 ± 0.047 | 0.4905 ± 0.041 |
| | MICE | 0.9660 ± 0.007 | 0.9444 ± 0.010 | 0.9014 ± 0.005 | 0.8532 ± 0.005 | 0.8041 ± 0.007 | 0.7350 ± 0.010 | 0.6445 ± 0.034 | 0.5782 ± 0.037 | 0.5256 ± 0.032 |
| | EM | 0.9631 ± 0.003 | 0.9262 ± 0.016 | 0.8582 ± 0.031 | 0.8223 ± 0.020 | 0.7798 ± 0.013 | 0.7407 ± 0.027 | 0.6848 ± 0.024 | 0.6099 ± 0.019 | 0.5529 ± 0.041 |
| | MisF | 0.9831 ± 0.008 | 0.9684 ± 0.012 | 0.9323 ± 0.015 | 0.8918 ± 0.017 | 0.8428 ± 0.018 | 0.7807 ± 0.015 | 0.7019 ± 0.012 | 0.6354 ± 0.022 | 0.5617 ± 0.023 |
| | GAIN | 0.9461 ± 0.026 | 0.9246 ± 0.008 | 0.8635 ± 0.029 | 0.8130 ± 0.019 | 0.7747 ± 0.025 | 0.7255 ± 0.023 | 0.6645 ± 0.026 | 0.5980 ± 0.025 | 0.5417 ± 0.026 |
| | genRBF | 0.9416 ± 0.004 | 0.9156 ± 0.008 | 0.8679 ± 0.010 | 0.8143 ± 0.015 | 0.7445 ± 0.034 | 0.6893 ± 0.030 | 0.6350 ± 0.047 | 0.5563 ± 0.042 | 0.4455 ± 0.062 |
| | KPCA | 0.9830 ± 0.008 | 0.9609 ± 0.006 | 0.9298 ± 0.020 | 0.8873 ± 0.019 | 0.8203 ± 0.037 | 0.7666 ± 0.031 | 0.7090 ± 0.013 | 0.6495 ± 0.017 | 0.5851 ± 0.039 |
| | PPCA | 0.9547 ± 0.020 | 0.9422 ± 0.012 | 0.8957 ± 0.017 | 0.8410 ± 0.014 | 0.7944 ± 0.022 | 0.7243 ± 0.020 | 0.6524 ± 0.015 | 0.5777 ± 0.034 | 0.5494 ± 0.040 |
| | HI- PMK | 0.9683 ± 0.011 | 0.9411 ± 0.021 | 0.8885 ± 0.023 | 0.8377 ± 0.010 | 0.7883 ± 0.023 | 0.7194 ± 0.021 | 0.6680 ± 0.015 | 0.6472 ± 0.015 | 0.5641 ± 0.038 |
| MAR | Mean | 0.9794 ± 0.006 | 0.9521 ± 0.010 | 0.9610 ± 0.007 | 0.8914 ± 0.015 | 0.9124 ± 0.008 | 0.7725 ± 0.029 | 0.9012 ± 0.014 | 0.7258 ± 0.033 | 0.5683 ± 0.014 |
| | MICE | 0.9779 ± 0.006 | 0.9490 ± 0.014 | 0.9601 ± 0.010 | 0.9265 ± 0.014 | 0.9126 ± 0.011 | 0.7562 ± 0.026 | 0.8881 ± 0.011 | 0.6953 ± 0.037 | 0.5488 ± 0.027 |
| | EM | 0.9757 ± 0.007 | 0.9322 ± 0.011 | 0.9499 ± 0.019 | 0.8664 ± 0.018 | 0.8701 ± 0.017 | 0.7382 ± 0.038 | 0.8737 ± 0.024 | 0.6717 ± 0.033 | 0.5514 ± 0.036 |
| | MisF | 0.9853 ± 0.005 | 0.9698 ± 0.008 | 0.9610 ± 0.009 | 0.8983 ± 0.015 | 0.9182 ± 0.006 | 0.7899 ± 0.014 | 0.8951 ± 0.021 | 0.6979 ± 0.014 | 0.5793 ± 0.025 |
| | GAIN | 0.9565 ± 0.010 | 0.9242 ± 0.019 | 0.9269 ± 0.003 | 0.8537 ± 0.042 | 0.8740 ± 0.032 | 0.7284 ± 0.036 | 0.8713 ± 0.037 | 0.6415 ± 0.030 | 0.5189 ± 0.019 |
| | genRBF | 0.9558 ± 0.018 | 0.9038 ± 0.014 | 0.9061 ± 0.033 | 0.8532 ± 0.021 | 0.8237 ± 0.019 | 0.7255 ± 0.022 | 0.7550 ± 0.019 | 0.7015 ± 0.015 | 0.6553 ± 0.021 |
| | KPCA | 0.9897 ± 0.004 | 0.9756 ± 0.008 | 0.9749 ± 0.016 | 0.9377 ± 0.007 | 0.9360 ± 0.014 | 0.7751 ± 0.025 | 0.8952 ± 0.013 | 0.7320 ± 0.028 | 0.6201 ± 0.024 |
| | PPCA | 0.9779 ± 0.006 | 0.9369 ± 0.023 | 0.9504 ± 0.014 | 0.9243 ± 0.016 | 0.9052 ± 0.015 | 0.7015 ± 0.027 | 0.8850 ± 0.009 | 0.6941 ± 0.037 | 0.5491 ± 0.028 |
| | HI- PMK | 0.9698 ± 0.008 | 0.9454 ± 0.016 | 0.9470 ± 0.009 | 0.9182 ± 0.010 | 0.8813 ± 0.014 | 0.7381 ± 0.029 | 0.8795 ± 0.011 | 0.6997 ± 0.033 | 0.5722 ± 0.043 |
| MNAR | Mean | 0.8848 ± 0.018 | 0.8724 ± 0.016 | 0.8335 ± 0.012 | 0.7877 ± 0.014 | 0.7193 ± 0.011 | 0.6606 ± 0.021 | 0.5758 ± 0.031 | 0.4390 ± 0.024 | 0.3962 ± 0.020 |
| | MICE | 0.9112 ± 0.013 | 0.8846 ± 0.017 | 0.8564 ± 0.022 | 0.8353 ± 0.025 | 0.7036 ± 0.022 | 0.6575 ± 0.015 | 0.5809 ± 0.028 | 0.4635 ± 0.026 | 0.4376 ± 0.030 |
| | EM | 0.9471 ± 0.016 | 0.9233 ± 0.013 | 0.8804 ± 0.017 | 0.8179 ± 0.026 | 0.7663 ± 0.016 | 0.7059 ± 0.005 | 0.6762 ± 0.035 | 0.5362 ± 0.040 | 0.5025 ± 0.025 |
| | MisF | 0.8804 ± 0.020 | 0.8409 ± 0.013 | 0.8373 ± 0.012 | 0.8049 ± 0.012 | 0.7410 ± 0.027 | 0.7022 ± 0.019 | 0.6330 ± 0.058 | 0.6030 ± 0.118 | 0.4573 ± 0.018 |
| | GAIN | 0.9141 ± 0.029 | 0.8831 ± 0.048 | 0.8371 ± 0.012 | 0.8529 ± 0.023 | 0.7835 ± 0.036 | 0.6933 ± 0.064 | 0.7379 ± 0.079 | 0.6331 ± 0.155 | 0.6037 ± 0.107 |
| | genRBF | 0.8439 ± 0.019 | 0.7860 ± 0.018 | 0.7967 ± 0.018 | 0.7562 ± 0.035 | 0.6606 ± 0.045 | 0.6242 ± 0.039 | 0.5099 ± 0.065 | 0.3990 ± 0.025 | 0.3745 ± 0.018 |
| | KPCA | 0.9941 ± 0.006 | 0.9882 ± 0.006 | 0.9757 ± 0.009 | 0.9331 ± 0.013 | 0.8963 ± 0.019 | 0.7990 ± 0.034 | 0.8202 ± 0.029 | 0.7879 ± 0.017 | 0.7357 ± 0.023 |
| | PPCA | 0.9614 ± 0.016 | 0.9533 ± 0.014 | 0.9081 ± 0.027 | 0.8516 ± 0.014 | 0.8025 ± 0.019 | 0.6838 ± 0.023 | 0.7268 ± 0.034 | 0.6486 ± 0.115 | 0.5873 ± 0.101 |
| | HI- PMK | 0.9322 ± 0.019 | 0.9183 ± 0.015 | 0.8760 ± 0.015 | 0.8357 ± 0.019 | 0.8118 ± 0.017 | 0.7233 ± 0.025 | 0.7865 ± 0.039 | 0.7981 ± 0.048 | 0.7458 ± 0.035 |

Table 11: Detailed F1 scores and standard deviation for the **Heart** dataset.

| Type | Model | 0.05 | 0.1 | 0.2 | 0.3 | 0.4 | 0.5 | 0.6 | 0.7 | 0.8 |
|---|---|---|---|---|---|---|---|---|---|---|
| MCAR | Mean | 0.7727 ± 0.060 | 0.7751 ± 0.047 | 0.7390 ± 0.065 | 0.7378 ± 0.061 | 0.7077 ± 0.028 | 0.6927 ± 0.067 | 0.6760 ± 0.056 | 0.6639 ± 0.061 | 0.4556 ± 0.024 |
| | MICE | 0.7798 ± 0.063 | 0.7898 ± 0.042 | 0.7647 ± 0.050 | 0.7833 ± 0.063 | 0.7639 ± 0.069 | 0.7504 ± 0.062 | 0.7117 ± 0.031 | 0.7219 ± 0.069 | 0.5994 ± 0.041 |
| | EM | 0.7768 ± 0.038 | 0.7396 ± 0.076 | 0.7692 ± 0.073 | 0.7179 ± 0.023 | 0.6645 ± 0.025 | 0.6205 ± 0.040 | 0.6095 ± 0.050 | 0.5172 ± 0.052 | 0.5501 ± 0.017 |
| | MisF | 0.7548 ± 0.059 | 0.7298 ± 0.077 | 0.7376 ± 0.039 | 0.7467 ± 0.018 | 0.7297 ± 0.049 | 0.7294 ± 0.036 | 0.6806 ± 0.044 | 0.6053 ± 0.066 | 0.5657 ± 0.069 |
| | GAIN | 0.7464 ± 0.058 | 0.7045 ± 0.032 | 0.6988 ± 0.074 | 0.6718 ± 0.046 | 0.7019 ± 0.067 | 0.6020 ± 0.073 | 0.4780 ± 0.057 | 0.4263 ± 0.045 | 0.4118 ± 0.034 |
| | genRBF | 0.7171 ± 0.036 | 0.6924 ± 0.036 | 0.6976 ± 0.060 | 0.6496 ± 0.036 | 0.6533 ± 0.036 | 0.5954 ± 0.036 | 0.6014 ± 0.036 | 0.5608 ± 0.036 | 0.4146 ± 0.036 |
| | KPCA | 0.8122 ± 0.048 | 0.8271 ± 0.048 | 0.7981 ± 0.047 | 0.8059 ± 0.064 | 0.8141 ± 0.053 | 0.7692 ± 0.071 | 0.7446 ± 0.042 | 0.7128 ± 0.070 | 0.5727 ± 0.041 |
| | PPCA | 0.7486 ± 0.056 | 0.7432 ± 0.047 | 0.7487 ± 0.069 | 0.7452 ± 0.055 | 0.7615 ± 0.079 | 0.7272 ± 0.056 | 0.6819 ± 0.044 | 0.6955 ± 0.047 | 0.5758 ± 0.068 |
| | HI- PMK | 0.7927 ± 0.045 | 0.7781 ± 0.049 | 0.7940 ± 0.056 | 0.7653 ± 0.044 | 0.7903 ± 0.049 | 0.7787 ± 0.090 | 0.7007 ± 0.055 | 0.7242 ± 0.036 | 0.6602 ± 0.046 |
| MAR | Mean | 0.7744 ± 0.054 | 0.7915 ± 0.037 | 0.7941 ± 0.068 | 0.7799 ± 0.055 | 0.7084 ± 0.029 | 0.7326 ± 0.058 | 0.7196 ± 0.068 | 0.6960 ± 0.061 | 0.7598 ± 0.071 |
| | MICE | 0.7950 ± 0.062 | 0.7950 ± 0.043 | 0.7864 ± 0.071 | 0.7798 ± 0.077 | 0.7971 ± 0.042 | 0.7498 ± 0.054 | 0.7204 ± 0.035 | 0.7619 ± 0.070 | 0.7801 ± 0.081 |
| | EM | 0.7663 ± 0.053 | 0.7973 ± 0.045 | 0.7573 ± 0.065 | 0.7175 ± 0.046 | 0.6737 ± 0.067 | 0.7144 ± 0.041 | 0.6257 ± 0.051 | 0.6766 ± 0.042 | 0.6767 ± 0.055 |
| | MisF | 0.7663 ± 0.094 | 0.7584 ± 0.054 | 0.7759 ± 0.052 | 0.7623 ± 0.063 | 0.7603 ± 0.061 | 0.7455 ± 0.027 | 0.7203 ± 0.059 | 0.7293 ± 0.062 | 0.7822 ± 0.056 |
| | GAIN | 0.7529 ± 0.073 | 0.7433 ± 0.052 | 0.7417 ± 0.079 | 0.7421 ± 0.076 | 0.6811 ± 0.034 | 0.6516 ± 0.064 | 0.6045 ± 0.048 | 0.6405 ± 0.090 | 0.6454 ± 0.053 |
| | genRBF | 0.6969 ± 0.004 | 0.7155 ± 0.004 | 0.7159 ± 0.004 | 0.7175 ± 0.004 | 0.6434 ± 0.004 | 0.6724 ± 0.004 | 0.6500 ± 0.004 | 0.7135 ± 0.004 | 0.7021 ± 0.004 |
| | KPCA | 0.7985 ± 0.038 | 0.7892 ± 0.034 | 0.7669 ± 0.074 | 0.7936 ± 0.061 | 0.8173 ± 0.035 | 0.7500 ± 0.088 | 0.7608 ± 0.032 | 0.7452 ± 0.090 | 0.8157 ± 0.049 |
| | PPCA | 0.7685 ± 0.081 | 0.7587 ± 0.048 | 0.7476 ± 0.052 | 0.7389 ± 0.097 | 0.7245 ± 0.069 | 0.6898 ± 0.042 | 0.6796 ± 0.066 | 0.6845 ± 0.100 | 0.7427 ± 0.087 |
| | HI- PMK | 0.8192 ± 0.069 | 0.8382 ± 0.042 | 0.8416 ± 0.078 | 0.8237 ± 0.068 | 0.8278 ± 0.057 | 0.7947 ± 0.052 | 0.7484 ± 0.057 | 0.8251 ± 0.071 | 0.7971 ± 0.098 |
| MNAR | Mean | 0.7641 ± 0.071 | 0.7595 ± 0.060 | 0.7096 ± 0.057 | 0.6560 ± 0.059 | 0.5352 ± 0.080 | 0.3960 ± 0.044 | 0.3459 ± 0.005 | 0.3480 ± 0.004 | 0.3480 ± 0.004 |
| | MICE | 0.7859 ± 0.052 | 0.7771 ± 0.045 | 0.7796 ± 0.062 | 0.7292 ± 0.049 | 0.6535 ± 0.077 | 0.4392 ± 0.069 | 0.3673 ± 0.044 | 0.3480 ± 0.004 | 0.3480 ± 0.004 |
| | EM | 0.7641 ± 0.049 | 0.7610 ± 0.077 | 0.7583 ± 0.065 | 0.7017 ± 0.102 | 0.6424 ± 0.087 | 0.5826 ± 0.094 | 0.4664 ± 0.065 | 0.3642 ± 0.041 | 0.3480 ± 0.004 |
| | MisF | 0.7758 ± 0.064 | 0.7716 ± 0.080 | 0.7284 ± 0.063 | 0.7240 ± 0.062 | 0.6882 ± 0.050 | 0.5636 ± 0.078 | 0.5364 ± 0.035 | 0.4495 ± 0.066 | 0.3570 ± 0.026 |
| | GAIN | 0.7361 ± 0.062 | 0.7725 ± 0.068 | 0.6954 ± 0.058 | 0.7113 ± 0.064 | 0.7013 ± 0.101 | 0.6555 ± 0.048 | 0.5210 ± 0.080 | 0.5188 ± 0.075 | 0.4605 ± 0.037 |
| | genRBF | 0.7883 ± 0.051 | 0.7677 ± 0.053 | 0.7797 ± 0.050 | 0.7075 ± 0.061 | 0.6742 ± 0.047 | 0.6058 ± 0.062 | 0.6885 ± 0.055 | 0.6274 ± 0.060 | 0.6364 ± 0.049 |
| | KPCA | 0.8178 ± 0.041 | 0.8172 ± 0.055 | 0.7939 ± 0.041 | 0.7859 ± 0.078 | 0.7265 ± 0.061 | 0.7020 ± 0.070 | 0.7273 ± 0.031 | 0.6779 ± 0.051 | 0.6755 ± 0.038 |
| | PPCA | 0.7495 ± 0.049 | 0.7294 ± 0.058 | 0.7335 ± 0.057 | 0.6669 ± 0.076 | 0.4894 ± 0.096 | 0.3480 ± 0.004 | 0.3480 ± 0.004 | 0.3480 ± 0.004 | 0.3480 ± 0.004 |
| | HI- PMK | 0.7636 ± 0.036 | 0.7778 ± 0.036 | 0.7674 ± 0.036 | 0.7853 ± 0.036 | 0.8226 ± 0.036 | 0.7983 ± 0.036 | 0.7870 ± 0.034 | 0.7258 ± 0.036 | 0.7358 ± 0.036 |

Table 12: Detailed F1 scores and standard deviation for the **Sonar** dataset.

| Type | Model | 0.05 | 0.1 | 0.2 | 0.3 | 0.4 | 0.5 | 0.6 | 0.7 | 0.8 |
|---|---|---|---|---|---|---|---|---|---|---|
| MCAR | Mean | 0.7886 ± 0.012 | 0.7706 ± 0.011 | 0.7576 ± 0.010 | 0.7552 ± 0.018 | 0.7296 ± 0.019 | 0.7129 ± 0.019 | 0.6636 ± 0.029 | 0.5836 ± 0.023 | 0.5188 ± 0.025 |
| | MICE | 0.7930 ± 0.013 | 0.7775 ± 0.013 | 0.7420 ± 0.010 | 0.7213 ± 0.015 | 0.7007 ± 0.023 | 0.6623 ± 0.018 | 0.6213 ± 0.020 | 0.6409 ± 0.019 | 0.5810 ± 0.021 |
| | EM | 0.6418 ± 0.013 | 0.6195 ± 0.015 | 0.5943 ± 0.026 | 0.5487 ± 0.025 | 0.4985 ± 0.038 | 0.4615 ± 0.038 | 0.4335 ± 0.031 | 0.4216 ± 0.021 | 0.4138 ± 0.030 |
| | MisF | 0.8401 ± 0.019 | 0.7078 ± 0.046 | 0.5723 ± 0.024 | 0.5022 ± 0.026 | 0.4891 ± 0.025 | 0.5080 ± 0.018 | 0.4949 ± 0.015 | 0.5011 ± 0.028 | 0.5093 ± 0.018 |
| | GAIN | 0.8862 ± 0.019 | 0.8828 ± 0.025 | 0.8674 ± 0.026 | 0.8699 ± 0.024 | 0.8428 ± 0.039 | 0.8246 ± 0.043 | 0.8101 ± 0.032 | 0.7746 ± 0.036 | 0.7579 ± 0.018 |
| | genRBF | 0.8644 ± 0.021 | 0.8557 ± 0.023 | 0.8456 ± 0.022 | 0.8340 ± 0.025 | 0.8196 ± 0.030 | 0.7956 ± 0.028 | 0.7589 ± 0.018 | 0.7185 ± 0.017 | 0.6524 ± 0.013 |
| | KPCA | 0.7958 ± 0.017 | 0.7821 ± 0.025 | 0.6749 ± 0.047 | 0.6319 ± 0.053 | 0.5722 ± 0.024 | 0.5771 ± 0.056 | 0.5936 ± 0.057 | 0.6052 ± 0.074 | 0.6177 ± 0.067 |
| | PPCA | 0.6594 ± 0.018 | 0.6518 ± 0.017 | 0.6324 ± 0.018 | 0.6155 ± 0.030 | 0.6169 ± 0.031 | 0.6073 ± 0.032 | 0.5365 ± 0.058 | 0.5337 ± 0.022 | 0.4648 ± 0.024 |
| | HI- PMK | 0.9339 ± 0.009 | 0.9222 ± 0.008 | 0.9080 ± 0.011 | 0.8935 ± 0.013 | 0.8750 ± 0.010 | 0.8622 ± 0.009 | 0.8401 ± 0.012 | 0.8067 ± 0.012 | 0.7639 ± 0.015 |
| MAR | Mean | 0.6648 ± 0.017 | 0.6352 ± 0.024 | 0.6160 ± 0.021 | 0.6052 ± 0.020 | 0.6715 ± 0.023 | 0.5282 ± 0.024 | 0.5195 ± 0.014 | 0.4788 ± 0.024 | 0.4602 ± 0.012 |
| | MICE | 0.6744 ± 0.017 | 0.6796 ± 0.023 | 0.6312 ± 0.031 | 0.6434 ± 0.023 | 0.6670 ± 0.025 | 0.6256 ± 0.017 | 0.6549 ± 0.010 | 0.6641 ± 0.036 | 0.4722 ± 0.037 |
| | EM | 0.6523 ± 0.019 | 0.6241 ± 0.017 | 0.5708 ± 0.033 | 0.5494 ± 0.024 | 0.6542 ± 0.016 | 0.4777 ± 0.046 | 0.4477 ± 0.025 | 0.4401 ± 0.029 | 0.4201 ± 0.058 |
| | MisF | 0.8664 ± 0.016 | 0.7760 ± 0.027 | 0.6227 ± 0.013 | 0.5666 ± 0.023 | 0.5274 ± 0.024 | 0.4998 ± 0.019 | 0.5016 ± 0.031 | 0.5000 ± 0.017 | 0.4924 ± 0.019 |
| | GAIN | 0.9128 ± 0.019 | 0.9085 ± 0.011 | 0.8881 ± 0.014 | 0.8926 ± 0.021 | 0.8546 ± 0.026 | 0.8605 ± 0.057 | 0.8432 ± 0.053 | 0.8368 ± 0.057 | 0.8013 ± 0.089 |
| | genRBF | 0.5046 ± 0.012 | 0.5074 ± 0.009 | 0.5052 ± 0.011 | 0.5140 ± 0.007 | 0.5068 ± 0.018 | 0.4975 ± 0.018 | 0.4946 ± 0.016 | 0.4849 ± 0.013 | 0.4863 ± 0.013 |
| | KPCA | 0.8145 ± 0.018 | 0.7889 ± 0.017 | 0.6676 ± 0.057 | 0.6271 ± 0.023 | 0.7402 ± 0.029 | 0.6228 ± 0.021 | 0.6680 ± 0.045 | 0.6763 ± 0.026 | 0.4873 ± 0.057 |
| | PPCA | 0.6661 ± 0.019 | 0.6601 ± 0.018 | 0.6251 ± 0.030 | 0.6356 ± 0.021 | 0.6561 ± 0.026 | 0.6224 ± 0.016 | 0.6230 ± 0.010 | 0.6465 ± 0.037 | 0.4714 ± 0.043 |
| | HI- PMK | 0.9336 ± 0.011 | 0.9321 ± 0.009 | 0.9163 ± 0.011 | 0.9059 ± 0.012 | 0.8989 ± 0.016 | 0.8991 ± 0.013 | 0.8852 ± 0.010 | 0.8825 ± 0.012 | 0.8324 ± 0.011 |
| MNAR | Mean | 0.8046 ± 0.013 | 0.8032 ± 0.014 | 0.7959 ± 0.015 | 0.7787 ± 0.013 | 0.7735 ± 0.014 | 0.7562 ± 0.014 | 0.7617 ± 0.015 | 0.7510 ± 0.022 | 0.7160 ± 0.012 |
| | MICE | 0.8046 ± 0.013 | 0.7959 ± 0.014 | 0.7710 ± 0.015 | 0.7456 ± 0.019 | 0.7384 ± 0.011 | 0.7057 ± 0.016 | 0.6692 ± 0.012 | 0.6699 ± 0.018 | 0.6790 ± 0.011 |
| | EM | 0.6684 ± 0.019 | 0.5971 ± 0.036 | 0.5190 ± 0.027 | 0.4787 ± 0.014 | 0.4639 ± 0.016 | 0.4560 ± 0.021 | 0.4500 ± 0.015 | 0.4330 ± 0.021 | 0.4226 ± 0.020 |
| | MisF | 0.9263 ± 0.017 | 0.9258 ± 0.017 | 0.9269 ± 0.017 | 0.9239 ± 0.018 | 0.9264 ± 0.017 | 0.9175 ± 0.014 | 0.9045 ± 0.021 | 0.8691 ± 0.013 | 0.7014 ± 0.049 |
| | GAIN | 0.8842 ± 0.040 | 0.9012 ± 0.047 | 0.9014 ± 0.039 | 0.9052 ± 0.048 | 0.9096 ± 0.045 | 0.9090 ± 0.047 | 0.9089 ± 0.033 | 0.9090 ± 0.045 | 0.8527 ± 0.050 |
| | genRBF | 0.8668 ± 0.020 | 0.8654 ± 0.021 | 0.8674 ± 0.022 | 0.8691 ± 0.021 | 0.8669 ± 0.021 | 0.8574 ± 0.023 | 0.8455 ± 0.021 | 0.8218 ± 0.021 | 0.7837 ± 0.018 |
| | KPCA | 0.8195 ± 0.018 | 0.7881 ± 0.023 | 0.7770 ± 0.019 | 0.7512 ± 0.015 | 0.7424 ± 0.023 | 0.7146 ± 0.025 | 0.6972 ± 0.027 | 0.7051 ± 0.022 | 0.7697 ± 0.069 |
| | PPCA | 0.6608 ± 0.023 | 0.6275 ± 0.025 | 0.5630 ± 0.030 | 0.5366 ± 0.025 | 0.5135 ± 0.024 | 0.4938 ± 0.025 | 0.4638 ± 0.018 | 0.5422 ± 0.055 | 0.5421 ± 0.035 |
| | HI- PMK | 0.9440 ± 0.009 | 0.9431 ± 0.010 | 0.9414 ± 0.010 | 0.9403 ± 0.012 | 0.9389 ± 0.011 | 0.9382 ± 0.009 | 0.9301 ± 0.014 | 0.9264 ± 0.014 | 0.9099 ± 0.010 |

Table 13: Detailed F1 scores and standard deviation for the **Spam** dataset.

| Type | Model | 0.05 | 0.1 | 0.2 | 0.3 | 0.4 | 0.5 | 0.6 | 0.7 | 0.8 |
|---|---|---|---|---|---|---|---|---|---|---|
| MCAR | Mean | 0.2439 ± 0.036 | 0.2416 ± 0.029 | 0.2391 ± 0.022 | 0.2298 ± 0.029 | 0.2159 ± 0.032 | 0.1990 ± 0.020 | 0.1581 ± 0.053 | 0.1400 ± 0.030 | 0.1191 ± 0.014 |
| | MICE | 0.2399 ± 0.032 | 0.2450 ± 0.034 | 0.2400 ± 0.023 | 0.2429 ± 0.036 | 0.2382 ± 0.036 | 0.2308 ± 0.028 | 0.1968 ± 0.038 | 0.1360 ± 0.030 | 0.1436 ± 0.037 |
| | EM | 0.1768 ± 0.008 | 0.1836 ± 0.014 | 0.1804 ± 0.013 | 0.1666 ± 0.012 | 0.1612 ± 0.025 | 0.1765 ± 0.008 | 0.1728 ± 0.011 | 0.1756 ± 0.005 | 0.1741 ± 0.026 |
| | MisF | 0.1961 ± 0.024 | 0.2116 ± 0.041 | 0.1757 ± 0.012 | 0.1905 ± 0.044 | 0.1686 ± 0.042 | 0.1681 ± 0.037 | 0.1497 ± 0.013 | 0.1204 ± 0.025 | 0.1134 ± 0.029 |
| | GAIN | 0.1901 ± 0.017 | 0.1803 ± 0.007 | 0.1763 ± 0.009 | 0.1695 ± 0.017 | 0.1764 ± 0.005 | 0.1628 ± 0.019 | 0.1762 ± 0.007 | 0.1781 ± 0.006 | 0.1936 ± 0.014 |
| | genRBF | 0.2500 ± 0.047 | 0.2469 ± 0.042 | 0.2552 ± 0.049 | 0.2475 ± 0.040 | 0.2265 ± 0.033 | 0.2241 ± 0.045 | 0.2022 ± 0.050 | 0.1745 ± 0.033 | 0.1486 ± 0.048 |
| | KPCA | 0.2607 ± 0.028 | 0.2615 ± 0.029 | 0.2448 ± 0.024 | 0.2414 ± 0.018 | 0.2231 ± 0.021 | 0.2296 ± 0.015 | 0.2121 ± 0.014 | 0.1978 ± 0.011 | 0.1855 ± 0.015 |
| | PPCA | 0.2456 ± 0.019 | 0.2451 ± 0.019 | 0.2428 ± 0.023 | 0.2423 ± 0.021 | 0.2376 ± 0.019 | 0.2312 ± 0.019 | 0.2215 ± 0.008 | 0.2016 ± 0.017 | 0.1852 ± 0.019 |
| | HI- PMK | 0.2584 ± 0.018 | 0.2571 ± 0.017 | 0.2517 ± 0.023 | 0.2515 ± 0.020 | 0.2319 ± 0.013 | 0.2323 ± 0.004 | 0.2334 ± 0.015 | 0.2062 ± 0.013 | 0.2044 ± 0.019 |
| MAR | Mean | 0.2443 ± 0.019 | 0.2367 ± 0.014 | 0.2427 ± 0.014 | 0.2442 ± 0.011 | 0.2293 ± 0.015 | 0.2327 ± 0.015 | 0.2342 ± 0.011 | 0.2104 ± 0.012 | 0.2215 ± 0.009 |
| | MICE | 0.2497 ± 0.018 | 0.2400 ± 0.016 | 0.2442 ± 0.013 | 0.2450 ± 0.013 | 0.2359 ± 0.016 | 0.2402 ± 0.015 | 0.2401 ± 0.018 | 0.2196 ± 0.025 | 0.2218 ± 0.012 |
| | EM | 0.1710 ± 0.009 | 0.1752 ± 0.017 | 0.1883 ± 0.016 | 0.1812 ± 0.019 | 0.1767 ± 0.013 | 0.1830 ± 0.021 | 0.1667 ± 0.021 | 0.1850 ± 0.019 | 0.1854 ± 0.006 |
| | MisF | 0.1863 ± 0.017 | 0.1903 ± 0.018 | 0.1939 ± 0.015 | 0.1867 ± 0.020 | 0.2050 ± 0.038 | 0.1766 ± 0.037 | 0.1913 ± 0.047 | 0.1447 ± 0.038 | 0.0603 ± 0.028 |
| | GAIN | 0.1888 ± 0.023 | 0.1913 ± 0.018 | 0.1940 ± 0.016 | 0.1766 ± 0.012 | 0.1963 ± 0.026 | 0.1875 ± 0.013 | 0.1740 ± 0.011 | 0.1582 ± 0.022 | 0.1897 ± 0.009 |
| | genRBF | 0.1867 ± 0.011 | 0.1824 ± 0.011 | 0.1819 ± 0.010 | 0.1774 ± 0.010 | 0.1842 ± 0.008 | 0.1759 ± 0.017 | 0.1783 ± 0.010 | 0.1795 ± 0.009 | 0.1547 ± 1924 |
| | KPCA | 0.2544 ± 0.020 | 0.2483 ± 0.024 | 0.2586 ± 0.026 | 0.2483 ± 0.016 | 0.2327 ± 0.014 | 0.2490 ± 0.016 | 0.2287 ± 0.006 | 0.2131 ± 0.017 | 0.2292 ± 0.018 |
| | PPCA | 0.2436 ± 0.018 | 0.2422 ± 0.014 | 0.2389 ± 0.013 | 0.2436 ± 0.015 | 0.2323 ± 0.016 | 0.2382 ± 0.015 | 0.2381 ± 0.016 | 0.2188 ± 0.027 | 0.2213 ± 0.010 |
| | HI- PMK | 0.2577 ± 0.020 | 0.2455 ± 0.010 | 0.2584 ± 0.011 | 0.2514 ± 0.008 | 0.2433 ± 0.007 | 0.2393 ± 0.008 | 0.2253 ± 0.013 | 0.2298 ± 0.013 | 0.2354 ± 0.014 |
| MNAR | Mean | 0.2452 ± 0.045 | 0.2353 ± 0.037 | 0.2305 ± 0.044 | 0.2207 ± 0.036 | 0.1949 ± 0.038 | 0.1924 ± 0.038 | 0.1882 ± 0.015 | 0.1782 ± 0.015 | 0.1791 ± 0.014 |
| | MICE | 0.1745 ± 0.042 | 0.1708 ± 0.035 | 0.1788 ± 0.039 | 0.1822 ± 0.040 | 0.1802 ± 0.022 | 0.1810 ± 0.026 | 0.1778 ± 0.026 | 0.1682 ± 0.053 | 0.1681 ± 0.032 |
| | EM | 0.1745 ± 0.007 | 0.1638 ± 0.007 | 0.1768 ± 0.012 | 0.1822 ± 0.018 | 0.1682 ± 0.019 | 0.1790 ± 0.017 | 0.1878 ± 0.006 | 0.1582 ± 0.021 | 0.1781 ± 0.025 |
| | MisF | 0.2013 ± 0.011 | 0.1940 ± 0.032 | 0.1735 ± 0.034 | 0.1692 ± 0.026 | 0.1751 ± 0.013 | 0.1836 ± 0.015 | 0.1860 ± 0.029 | 0.1810 ± 0.031 | 0.1502 ± 0.028 |
| | GAIN | 0.1977 ± 0.014 | 0.1770 ± 0.015 | 0.1744 ± 0.016 | 0.1872 ± 0.022 | 0.1864 ± 0.018 | 0.1737 ± 0.009 | 0.1843 ± 0.017 | 0.1718 ± 0.014 | 0.1727 ± 0.015 |
| | genRBF | 0.2312 ± 0.010 | 0.2273 ± 0.014 | 0.2195 ± 0.017 | 0.2107 ± 0.021 | 0.1899 ± 0.012 | 0.1904 ± 0.017 | 0.1982 ± 0.014 | 0.1882 ± 0.047 | 0.1891 ± 0.019 |
| | KPCA | 0.2450 ± 0.009 | 0.2436 ± 0.026 | 0.2428 ± 0.019 | 0.2368 ± 0.013 | 0.2287 ± 0.017 | 0.2311 ± 0.016 | 0.2171 ± 0.015 | 0.2110 ± 0.012 | 0.1916 ± 0.006 |
| | PPCA | 0.2431 ± 0.018 | 0.2361 ± 0.023 | 0.2376 ± 0.015 | 0.2362 ± 0.020 | 0.2302 ± 0.006 | 0.2199 ± 0.009 | 0.1975 ± 0.017 | 0.1887 ± 0.006 | 0.1738 ± 0.027 |
| | HI- PMK | 0.2455 ± 0.011 | 0.2510 ± 0.011 | 0.2522 ± 0.016 | 0.2337 ± 0.012 | 0.2318 ± 0.009 | 0.2153 ± 0.005 | 0.2051 ± 0.012 | 0.2135 ± 0.011 | 0.2125 ± 0.003 |

Table 14: Detailed F1 scores and standard deviation for the **Student** dataset.

| Type | Model | 0.05 | 0.1 | 0.2 | 0.3 | 0.4 | 0.5 | 0.6 | 0.7 | 0.8 |
|---|---|---|---|---|---|---|---|---|---|---|
| MCAR | Mean | 0.8949 ± 0.010 | 0.8824 ± 0.010 | 0.8674 ± 0.013 | 0.8477 ± 0.010 | 0.8204 ± 0.009 | 0.7854 ± 0.009 | 0.7443 ± 0.011 | 0.6947 ± 0.016 | 0.6287 ± 0.008 |
| | MICE | 0.9109 ± 0.011 | 0.9118 ± 0.009 | 0.9065 ± 0.013 | 0.8908 ± 0.011 | 0.8904 ± 0.005 | 0.8555 ± 0.005 | 0.8347 ± 0.006 | 0.7943 ± 0.010 | 0.7120 ± 0.011 |
| | EM | 0.8800 ± 0.011 | 0.8639 ± 0.010 | 0.8190 ± 0.013 | 0.7753 ± 0.006 | 0.7352 ± 0.007 | 0.6807 ± 0.014 | 0.5959 ± 0.033 | 0.4298 ± 0.000 | 0.4298 ± 0.000 |
| | MisF | 0.9823 ± 0.006 | 0.9835 ± 0.004 | 0.9798 ± 0.005 | 0.9751 ± 0.007 | 0.9602 ± 0.007 | 0.9307 ± 0.004 | 0.9003 ± 0.014 | 0.8423 ± 0.017 | 0.7566 ± 0.015 |
| | GAIN | 0.9669 ± 0.006 | 0.9586 ± 0.006 | 0.9432 ± 0.005 | 0.9117 ± 0.011 | 0.8864 ± 0.013 | 0.8527 ± 0.015 | 0.8102 ± 0.007 | 0.7088 ± 0.031 | 0.5783 ± 0.015 |
| | genRBF | 0.9823 ± 0.005 | 0.9761 ± 0.006 | 0.9545 ± 0.006 | 0.9379 ± 0.003 | 0.9096 ± 0.005 | 0.8789 ± 0.007 | 0.8345 ± 0.007 | 0.7779 ± 0.010 | 0.6925 ± 0.007 |
| | KPCA | 0.9229 ± 0.009 | 0.9198 ± 0.009 | 0.9111 ± 0.008 | 0.8908 ± 0.008 | 0.8850 ± 0.007 | 0.8594 ± 0.014 | 0.8404 ± 0.015 | 0.8008 ± 0.011 | 0.7185 ± 0.019 |
| | PPCA | 0.8931 ± 0.008 | 0.8791 ± 0.010 | 0.8455 ± 0.009 | 0.8059 ± 0.010 | 0.7726 ± 0.014 | 0.7353 ± 0.015 | 0.6960 ± 0.014 | 0.6454 ± 0.017 | 0.5825 ± 0.013 |
| | HI-PMK | 0.9919 ± 0.003 | 0.9906 ± 0.002 | 0.9869 ± 0.002 | 0.9782 ± 0.004 | 0.9628 ± 0.006 | 0.9393 ± 0.005 | 0.9073 ± 0.008 | 0.8577 ± 0.015 | 0.7812 ± 0.012 |
| MAR | Mean | 0.9046 ± 0.010 | 0.8325 ± 0.014 | 0.8466 ± 0.013 | 0.8193 ± 0.012 | 0.8281 ± 0.006 | 0.9005 ± 0.012 | 0.6848 ± 0.028 | 0.6113 ± 0.015 | 0.5741 ± 0.014 |
| | MICE | 0.9074 ± 0.008 | 0.9020 ± 0.005 | 0.9004 ± 0.008 | 0.8815 ± 0.008 | 0.8954 ± 0.005 | 0.9032 ± 0.011 | 0.8127 ± 0.010 | 0.8363 ± 0.025 | 0.6251 ± 0.037 |
| | EM | 0.8858 ± 0.010 | 0.8435 ± 0.008 | 0.8216 ± 0.011 | 0.7577 ± 0.017 | 0.8050 ± 0.008 | 0.8945 ± 0.012 | 0.5937 ± 0.014 | 0.4298 ± 0.000 | 0.4298 ± 0.000 |
| | MisF | 0.9823 ± 0.006 | 0.9819 ± 0.005 | 0.9780 ± 0.005 | 0.9773 ± 0.003 | 0.9708 ± 0.003 | 0.9705 ± 0.007 | 0.9097 ± 0.013 | 0.9015 ± 0.016 | 0.8510 ± 0.016 |
| | GAIN | 0.9651 ± 0.008 | 0.9622 ± 0.006 | 0.9586 ± 0.007 | 0.9428 ± 0.011 | 0.9078 ± 0.027 | 0.9403 ± 0.018 | 0.8195 ± 0.016 | 0.8533 ± 0.006 | 0.8194 ± 0.013 |
| | genRBF | 0.8816 ± 0.007 | 0.8706 ± 0.007 | 0.8340 ± 0.011 | 0.8512 ± 0.007 | 0.8161 ± 0.005 | 0.8554 ± 0.010 | 0.7713 ± 0.004 | 0.7822 ± 0.009 | 0.7489 ± 0.007 |
| | KPCA | 0.9239 ± 0.010 | 0.9217 ± 0.009 | 0.9147 ± 0.007 | 0.8936 ± 0.003 | 0.9059 ± 0.010 | 0.9089 ± 0.012 | 0.8515 ± 0.013 | 0.8621 ± 0.014 | 0.7762 ± 0.012 |
| | PPCA | 0.8983 ± 0.013 | 0.8821 ± 0.011 | 0.8402 ± 0.012 | 0.8557 ± 0.013 | 0.8241 ± 0.009 | 0.8947 ± 0.011 | 0.6870 ± 0.030 | 0.6165 ± 0.015 | 0.5725 ± 0.014 |
| | HI-PMK | 0.9921 ± 0.002 | 0.9923 ± 0.002 | 0.9854 ± 0.003 | 0.9838 ± 0.004 | 0.9750 ± 0.006 | 0.9741 ± 0.005 | 0.9205 ± 0.007 | 0.9176 ± 0.008 | 0.8781 ± 0.019 |
| MNAR | Mean | 0.8855 ± 0.011 | 0.8905 ± 0.012 | 0.8889 ± 0.017 | 0.8379 ± 0.006 | 0.7590 ± 0.015 | 0.6411 ± 0.022 | 0.5788 ± 0.024 | 0.5334 ± 0.023 | 0.4978 ± 0.016 |
| | MICE | 0.8996 ± 0.015 | 0.8814 ± 0.012 | 0.8448 ± 0.017 | 0.8148 ± 0.013 | 0.7816 ± 0.015 | 0.6051 ± 0.021 | 0.5839 ± 0.020 | 0.5721 ± 0.033 | 0.5577 ± 0.025 |
| | EM | 0.8513 ± 0.010 | 0.7746 ± 0.016 | 0.5534 ± 0.025 | 0.4479 ± 0.010 | 0.4318 ± 0.004 | 0.4298 ± 0.000 | 0.4298 ± 0.000 | 0.4298 ± 0.000 | 0.4298 ± 0.000 |
| | MisF | 0.9767 ± 0.004 | 0.9634 ± 0.002 | 0.9443 ± 0.003 | 0.9265 ± 0.010 | 0.8918 ± 0.005 | 0.8543 ± 0.010 | 0.8142 ± 0.017 | 0.7563 ± 0.014 | 0.6645 ± 0.033 |
| | GAIN | 0.9563 ± 0.019 | 0.9371 ± 0.038 | 0.9052 ± 0.060 | 0.8907 ± 0.044 | 0.8428 ± 0.074 | 0.8125 ± 0.054 | 0.8432 ± 0.053 | 0.8108 ± 0.034 | 0.6900 ± 0.090 |
| | genRBF | 0.9700 ± 0.003 | 0.9517 ± 0.004 | 0.9252 ± 0.006 | 0.8817 ± 0.011 | 0.8222 ± 0.018 | 0.7673 ± 0.020 | 0.7273 ± 0.019 | 0.6475 ± 0.023 | 0.5725 ± 0.025 |
| | KPCA | 0.9211 ± 0.008 | 0.9114 ± 0.018 | 0.8710 ± 0.013 | 0.8281 ± 0.020 | 0.7832 ± 0.022 | 0.6841 ± 0.008 | 0.7031 ± 0.018 | 0.7776 ± 0.038 | 0.7508 ± 0.055 |
| | PPCA | 0.9098 ± 0.010 | 0.9118 ± 0.010 | 0.8895 ± 0.013 | 0.8610 ± 0.015 | 0.8652 ± 0.014 | 0.8507 ± 0.010 | 0.8206 ± 0.013 | 0.7841 ± 0.014 | 0.7422 ± 0.014 |
| | HI-PMK | 0.9904 ± 0.004 | 0.9867 ± 0.004 | 0.9721 ± 0.003 | 0.9487 ± 0.002 | 0.9042 ± 0.004 | 0.8618 ± 0.004 | 0.8077 ± 0.017 | 0.8507 ± 0.024 | 0.8779 ± 0.014 |

Table 15: Detailed F1 scores and standard deviation for the **Wine** dataset.

# References

[1] Sunil Aryal, Kai Ming Ting, Takashi Washio, and Gholamreza Haffari. A comparative study of data-dependent approaches without learning in measuring similarities of data objects. *Data mining and knowledge discovery*, 34(1):124–162, 2020.

[2] Peter J. Huber and Elvezio M. Ronchetti. *Robust Statistics*. Wiley, Hoboken, NJ, 2 edition, 2009.

[3] Herbert A. Sturges. The choice of a class interval. *Journal of the American Statistical Association*, 21(153):65–66, 1926.

[4] Youran Zhou, Mohamed Reda Bouadjenek, Jonathan Wells, and Sunil Aryal. Hi-pmk: A data-dependent kernel for incomplete heterogeneous data representation, 2025.
